# Supplementary material for: Phase Separation Kinetics in a Polar Active Field Model
Source: arXiv:2508.13888 ancillary file (2025-08-19)
Supplement: Supplementary file 1 [file supplemental.pdf]

# Phase Separation Kinetics in a Polar Active Field Model
# Supplemental Material


Massimiliano Semeraro,[1,2,*] Leticia F. Cugliandolo,[3] Giuseppe Gonnella,[1,2] and Adriano Tiribocchi[4,5,†]

[1] *Dipartimento Interateneo di Fisica, Università degli Studi di Bari, via Amendola 173, Bari, I-70126, Italy*
[2] *INFN, Sezione di Bari, via Amendola 173, Bari, I-70126, Italy*
[3] *Sorbonne Université, Laboratoire de Physique Théorique et Hautes Energies, CNRS-UMR 7589, 4 Place Jussieu, 75252 Paris Cedex 05, France*
[4] *Istituto per le Applicazioni del Calcolo, Consiglio Nazionale delle Ricerche, Via dei Taurini 19, Rome, I-00185, Italy*
[5] *INFN Tor Vergata, Via della ricerca scientifica 1, Rome, I-00133, Italy*



(Dated: August 12, 2025)



The present document is the Supplemental Material for the paper *Phase Separation Kinetics in a Polar Active Field Model*. We develop further the description of the model, giving additional details on symmetries and properties of the structure factor and topological defects. We also thoroughly discuss functional descriptions of the stationary density and polarization fields and we give an argument for the faster growth found under sufficiently strong advection. We discuss how generalizations of the original model inspired by further continuous models affect the system morphology and domain growth. Finally, we provide details on the movies attached to the paper.


## CONTENTS


I. The Model 2
A. Free energy and equations of motion 2
B. Density and polarization at equilibrium 2

II. Numerical Methods 3
A. Simulation details 3
B. Cluster and defect identification 4

III. Polarization field around topological defects 5

IV. Morphology 5

V. The growing length 8

VI. Structure Factor and Dynamical Scaling 9

VII. Stationary density and polarization profiles of a single droplet 12
A. The stationary density and polarization profiles in the bulk 12
B. Stationary profile including the interface 16

VIII. An argument to explain the growth of $L(t)$ 17

IX. Morphology and domain growth in generalized models 20
A. Self-advection of the polarization 20
B. Contact with Active Model B 22
C. Additional splay contribution 24

X. Movies 26

References 27

# I. THE MODEL

## A. Free energy and equations of motion

Here we shortly outline the theoretical model of this work. We consider a two-dimensional system with periodic boundary conditions comprising a scalar field $\phi$ accounting for the local density and a vector polar field $\boldsymbol{p}$ capturing the local orientation of the active component. The system undergoes phase separation, with the polarization being slaved to the dense phase. The equilibrium properties of the mixture are described by the free energy functional

$$F[\phi,\boldsymbol{p}] = \int d^2x \, \left\{ \left[ \frac{\alpha_\phi}{4\phi_{cr}} \phi^2(\phi-\phi_0)^2 + \frac{k_\phi}{2}|\nabla\phi|^2 \right] + \left[ -\frac{\alpha_{\boldsymbol{p}}}{2}\frac{\phi-\phi_{cr}}{\phi_{cr}}|\boldsymbol{p}|^2 + \frac{\alpha_{\boldsymbol{p}}}{4}|\boldsymbol{p}|^4 + \frac{k_{\boldsymbol{p}}}{2}(\nabla\boldsymbol{p})^2 \right] \right\} \;, \tag{1}$$

where dependencies of $\phi$ and $\boldsymbol{p}$ on $\boldsymbol{r}$ and $t$ are implicit.

The first two terms are borrowed from a binary fluid formalism and account for bulk and interfacial properties of the mixture. More specifically, the double well potential $\alpha_\phi\phi^2(\phi-\phi_0)^2/4\phi_{cr}$ ensures the existence of two coexisting minima at $\phi = 0$ (dilute phase) and $\phi = \phi_0$ (dense phase), while the term $k_\phi|\nabla\phi|^2/2$ accounts for the energetic penalty due to the fluid interface. Also, the parameters $\alpha_\phi$ and $k_\phi$ are positive constants controlling surface tension and interface width, defined as $\sigma = \sqrt{8\alpha_\phi k_\phi/9}$ and $\xi = \sqrt{2k_\phi/\alpha_\phi}$ respectively [1].

The further three contributions to Eq. (1) stem from the liquid crystal formalism and are designed following an approach akin to the case of $\phi$. The two terms $-\alpha_{\boldsymbol{p}}(\phi-\phi_{cr})|\boldsymbol{p}|^2/(2\phi_{cr})+\alpha_{\boldsymbol{p}}|\boldsymbol{p}|^4/4$ individuate a quartic potential, with $|\boldsymbol{p}|$ denoting the modulus of the vector $\boldsymbol{p}$. Here $\phi_{cr} = \phi_0/2$ is the critical concentration at which the isotropic-to-polar transition occurs. We set $\phi_0 = 2$, thus $\phi_{cr} = 1$. Note that, if $\phi < \phi_{cr}$, the potential is a quartic parabola with minimum at 0, while if $\phi > \phi_{cr}$ it is half a double well with minimum at $\sqrt{(\phi-\phi_{cr})/\phi_{cr}}$. Hence, the polarization is slaved to the dense phase. Finally, the term $(k_{\boldsymbol{p}}/2)(\nabla\boldsymbol{p})^2 \equiv (k_{\boldsymbol{p}}/2)(\sum_{ij}\partial p_i/\partial r_j)^2$ ($i,j = 1,2$ dimensional indices) captures spatially inhomogeneous deformations of the polar field and corresponds to the single elastic constant approximation [2, 3].

The dynamics of the system is governed by the equations

$$\dot{\phi} + \lambda\nabla\cdot(\boldsymbol{p}\phi) = M\nabla^2\mu_\phi \;, \tag{2}$$

$$\dot{\boldsymbol{p}} = -\Gamma\boldsymbol{\mu}_{\boldsymbol{p}} \;, \tag{3}$$

where $M$ is the mobility, $\lambda$ is a positive paramter gauging the strength of the advective term and $\Gamma$ is the rotational viscosity. The functions $\mu_\phi$ and $\boldsymbol{\mu}_{\boldsymbol{p}}$ are the chemical potential and the molecular field, and are given by

$$\mu_\phi = \frac{\delta F}{\delta\phi} = \alpha_\phi(\phi^3 - 3\phi^2 + 2\phi) - k_\phi\nabla^2\phi - \frac{\alpha_p}{2}|\boldsymbol{p}|^2 \;, \tag{4}$$

and

$$\boldsymbol{\mu}_{\boldsymbol{p}} = \frac{\delta F}{\delta\boldsymbol{p}} = \alpha_p|\boldsymbol{p}|^2\cdot\boldsymbol{p} - \alpha_p(\phi-1)\boldsymbol{p} - k_p\nabla^2\boldsymbol{p} \;. \tag{5}$$

We also remark that an incompressibility-like condition typical of hydrodynamic theories, where $\nabla\cdot\boldsymbol{v} = 0$ for the velocity field $\boldsymbol{v}$, does not hold for $\boldsymbol{p}$ in this model.

Finally, as a benchmark test, in Fig. S1 we numerically show that, in agreement with Eq. (2), the total mass is conserved throughout the simulation for different values of initial concentration of the dense phase.

## B. Density and polarization at equilibrium

The equilibrium values of density and polarization, denoted as $\phi_{eq}$ and $|\boldsymbol{p}|_{eq}$, can be found by minimizing Eq. (1) neglecting all gradient contributions. This leads to the following equations

$$\frac{\delta F}{\delta\phi} = \frac{\alpha_\phi}{\phi_{cr}^4}\phi^3 - \frac{3}{2}\frac{\alpha_\phi\phi_0}{\phi_{cr}^4}\phi^2 + \frac{a\phi_0^2}{2\phi_{cr}^4}\phi - \frac{\alpha_{\boldsymbol{p}}}{2\phi_{cr}}|\boldsymbol{p}| = 0 \;, \tag{6}$$

$$\frac{\delta F}{\delta|\boldsymbol{p}|} = \alpha_p|\boldsymbol{p}|^3 - \frac{\alpha_p(\phi-\phi_{cr})}{\phi_{cr}}|\boldsymbol{p}| = 0 \;. \tag{7}$$

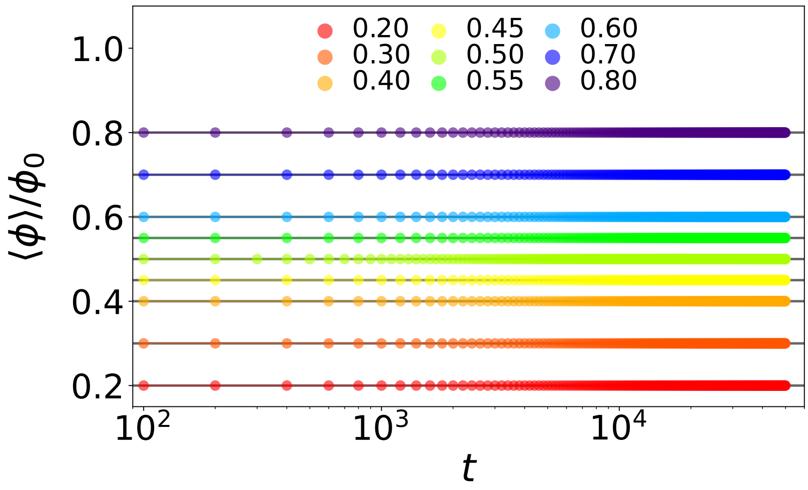


Figure S1. Numerical verification of mass conservation. Here $\langle\phi\rangle \equiv (\int_S d^2x\,\phi)/S$, where $S$ is the surface of the system where the integral is computed. Different colors correspond to the initial concentrations of the dense phase while the horizontal black lines are guides-to-the-eye. The system undergoes phase separation on a square lattice of linear size $N = 512$, while the parameters are $\phi_0 = 2$, $M = 1$, $\alpha_\phi = 0.1$, $k_\phi = 0.5$, $\Gamma = 1$, $\alpha_{\boldsymbol{p}} = 0.1$, $k_{\boldsymbol{p}} = 0.04$ and $\lambda = 10^{-2}$. See Sec. IIA for further details on initialization and numerical integration.

Using $\phi_{cr} = \phi_0/2$, besides $\phi_{eq} = 0$ and $|\boldsymbol{p}|_{eq} = 0$, non-trivial solutions are

$$\phi_{eq} = \frac{\phi_0}{2}\left(1 + \sqrt{1 + \frac{\alpha_{\boldsymbol{p}}}{2\alpha_\phi}}\right) , \tag{8}$$

$$|\boldsymbol{p}|_{eq} = \left(1 + \frac{\alpha_{\boldsymbol{p}}}{2\alpha_\phi}\right)^{\frac{1}{4}} , \tag{9}$$

in agreement with the ones obtained in [4].

## II. NUMERICAL METHODS

Eqs. (2) and (3) are integrated by using a finite-difference scheme, where differential operators are computed by standard stencil techniques [5]. Simulations are run on two-dimensional lattices of linear size $N$ ranging from 128 to 1024. In the following, we provide further details about the simulations of a phase-separated mixture and an isolated droplet as well as the procedures we use to implement clusters and to locate and identify topological defects.

### A. Simulation details

*Phase separation.* We initialized the simulation in a disordered state, i.e. $\phi(\mathbf{r}, 0) = \phi_{in} + \delta\phi(\mathbf{r}, 0)$ where $\phi_{in} = \phi_{cr}$ and $\delta\phi$ is a small perturbation extracted uniformly from $[-0.1, 0.1]$, while $\boldsymbol{p}$ is randomly oriented and has unitary modulus. The values of the thermodynamic parameters are $\alpha_\phi = 0.1$ and $k_\phi = 0.5$ which lead to $\sigma \sim 0.21$ and $\xi \sim 3.16$, $M = 1$, $\alpha_{\boldsymbol{p}} = 0.1$, $k_{\boldsymbol{p}} = 0.04$ and $\Gamma = 1$. Our simulations were run up to $10^7$ iterations on square lattices of linear size $N$ taking values 128, 256, 512 and 1024, with particular focus on the cases $N = 512$ and $N = 1024$. Also, we fixed lattice spacing $\Delta N = 1$ and time step $\Delta t = 10^{-2}$, although we verified that our results are numerically stable upon decreasing $\Delta N$ and $\Delta t$. Time and space are thus discretized as $t = n\Delta t$, with $n$ the iteration index, and $x = n_x\Delta N$, $y = n_y\Delta N$, with $n_x, n_y$ horizontal and vertical node indices. An approximate mapping between our simulations and a real system can be built following [6, 7], where length and time are rescaled by interface width $\xi = \sqrt{2k_\phi/\alpha_\phi}$ and interface diffusion time $t_D = \xi^3\phi_{eq}^2/(M\sigma)$ obtained from the relaxation of a planar interface separating two coexisting phases in the passive model B (i.e. with $\lambda = 0$ and $\boldsymbol{p} = 0$), with equilibrium profile $\phi(x) = \phi_{eq}\tanh(2x/\xi)$ and $\phi_{eq}$ being the equilibrium value of $\phi$ of the dense phase.

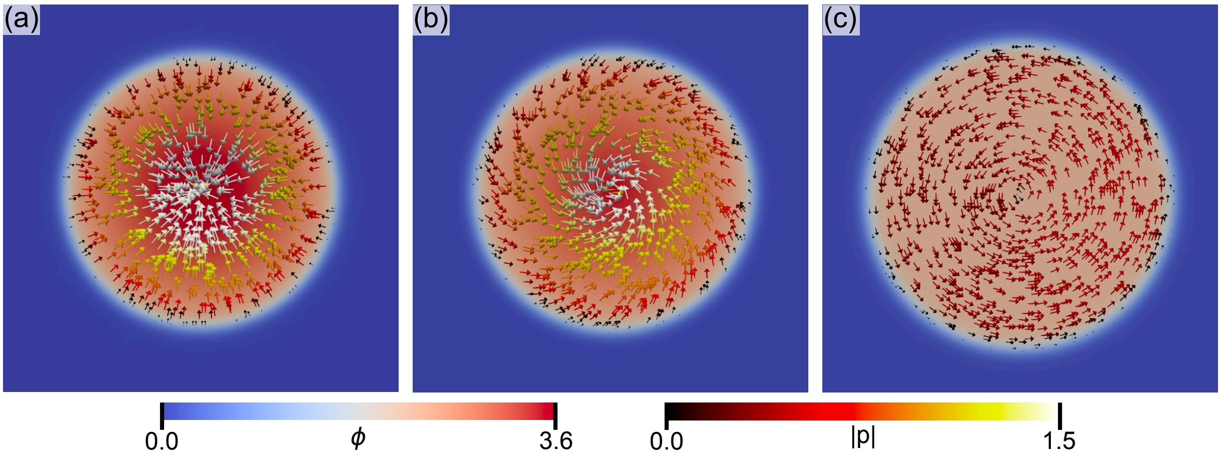


Figure S2. Snapshots of a circular droplet with an inward-aster-like (a), a spiral-like (b) and a vortex-like (c) polarization. In the spiral-like droplet, polarization vectors have a $\pi/4$ radial inclination. All droplets were obtained with $\lambda = 10^{-2}$, and have a radius $R \sim 45$, while the other parameters were fixed as detailed in the text. The background color represents the density $\phi$ according to the color map, while arrows represent instead polarization vectors, whose modulus is given by corresponding color map of $|\boldsymbol{p}|$.

The characteristic domain size $L(t)$ was evaluated as the inverse of the first moment of the normalized spherically-averaged structure factor [8, 9]

$$L(t) \equiv \pi \, \frac{\int dk \; S(k,t)}{\int dk \; kS(k,t)} \; , \tag{10}$$

where $k = |\boldsymbol{k}|$ is the modulus of the wave vector $\boldsymbol{k}$ in the Fourier space. The spherically-averaged structure factor is defined as

$$S(k,t) \equiv \langle \phi(\boldsymbol{k},t)\phi(-\boldsymbol{k},t)\rangle_k \; , \tag{11}$$

where $\phi(\boldsymbol{k},t)$ is the spatial Fourier transform of the density field $\phi$ and $\langle \ldots \rangle_k$ denotes an average over a shell in $\boldsymbol{k}$ space at fixed $k$.

*Isolated droplets.* In this case, circular droplets of initial radius ranging from $R \sim 10$ to $R \sim 250$ lattice sites are initially placed at the center of a square lattice, with $\phi = 2$ inside the droplets and zero outside, while the polarization is assigned a unit modulus inside the droplets and zero outside (see Fig. S2 for sample droplets with $R \sim 45$). We have considered three different initial orientations of $\boldsymbol{p}$, i.e. an aster-like poiting inwards (a), a spiral-like (b) and a vortex structure (c). The parameters are the same as the ones of the phase separation, and a typical simulation was run for $\sim 10^6$ time-steps.

### B. Cluster and defect identification

Cluster identification was performed using the Python-implemented DBSCAN algorithm [10]. In particular, we focused on regions of the system where $\phi \gtrsim 2$ and we considered two nodes of the lattice as being part of the same cluster if their distance is less than $1.5\Delta N$. We fixed to two the minimum number of close nodes that form a cluster. Once clusters were identified, their centers of mass were obtained as averages of the location of cluster lattice nodes weighted by the value of $\phi$ at each node. The cluster area was computed from the number of lattice nodes occupied by the domain while the cluster perimeter was estimated as the number of lattice nodes at the boundary of the cluster.

Topological defects are located where the polarization is null [2]. Thus, their location can be determined according to where $\nabla \cdot \boldsymbol{p}$ is most negative, which denotes a fast local decrease in the modulus of $\boldsymbol{p}$. Defects are then identified by computing the circulation of $\boldsymbol{p}$ over closed paths $\boldsymbol{\mathcal{C}}$ around the defect location. In Fig. S2, the circulation is null for aster-like configurations and non-zero for vortex-like ones (positive for counter-clockwise and negative for clockwise ones). Intermediate values identify spiral-like configurations. More in detail, once the maximum positive and negative values of circuitation for domains with defects in given configurations are determined, we identify as aster- and vortex-domains the ones whose circuitation (magnitude) is respectively lower and larger than 0.2 and 0.8 times the maximum values, while all other configurations are categorized as spirals.

## III. POLARIZATION FIELD AROUND TOPOLOGICAL DEFECTS

In Cartesian coordinates, two-dimensional aster-like, vortex-like and spiral-like configurations with center in the origin of the system (as the ones in Fig. S2) are described by the following polarization fields

$$\boldsymbol{p}_a(x,y) = \left( a_r(x,y)\frac{x}{\sqrt{x^2+y^2}},\ a_r(x,y)\frac{y}{\sqrt{x^2+y^2}} \right) , \tag{12}$$

$$\boldsymbol{p}_v(x,y) = \left( -a_\theta(x,y)\frac{y}{\sqrt{x^2+y^2}},\ a_\theta(x,y)\frac{x}{\sqrt{x^2+y^2}} \right) , \tag{13}$$

and

$$\boldsymbol{p}_s(x,y) = \boldsymbol{p}_a(x,y) + \boldsymbol{p}_v(x,y) , \tag{14}$$

where $a_r(x,y)$ and $a_\theta(x,y)$ represent the magnitude of the polar vectors in aster-like and vortex-like configurations, respectively, while the magnitude of the spiral-like configuration is given by $\sqrt{a_r^2(x,y)+a_\theta^2(x,y)}$.

In polar coordinates $(r,\theta)$, these expressions become

$$\boldsymbol{p}_a(r,\theta) = (p_r(r,\theta) = a(r,\theta),\quad p_\theta(r,\theta) = 0) , \tag{15}$$

$$\boldsymbol{p}_v(r,\theta) = (p_r(r,\theta) = 0,\quad p_\theta(r,\theta) = a_\theta(r,\theta)) , \tag{16}$$

$$\boldsymbol{p}_s(r,\theta) = (p_r(r,\theta) = a_r(r,\theta),\quad p_\theta(r,\theta) = a_\theta(r,\theta)) , \tag{17}$$

with $p_r(r,\theta)$ and $p_\theta(r,\theta)$ radial and tangential components of the polarization vector field. For aster-like configurations $a_r(r,\theta) < 0$ ($a_r(r,\theta) > 0$) corresponds to inward- (outward-) configurations, while for vortex-like configurations $a_\theta(r,\theta) < 0$ ($a_\theta(r,\theta) > 0$) corresponds to counter-clockwise (clockwise) ones.

For Eqs. (12)-(17) the winding number

$$w \equiv \frac{1}{2\pi}\int_{\boldsymbol{\mathcal{C}}} \nabla\theta(x,y)\cdot d\boldsymbol{\mathcal{C}} , \tag{18}$$

with $\theta(x,y) = \arctan\left(p_i^y(x,y)/p_i^x(x,y)\right)$ ($i = a, v, s$) local polarization orientation and $\boldsymbol{\mathcal{C}}$ any path closed around the defect core having counter-clockwise orientation, is equal to $+1$.

## IV. MORPHOLOGY

In this section, we provide further details about the domain morphology for different values of $\lambda$.

*Morphological evolution.* In Fig. S3 we show the time evolution of the active mixture for $\lambda = 10^{-4}$ (a), $\lambda = 10^{-3}$ (b), $\lambda = 10^{-2}$ (c) and $\lambda = 10^{-1}$ (d) (see also Movie S1 and S2). With reference to Fig. 2 of the main text, configurations (i) are taken approximately at $t \sim 10^3$ (i.e. after the initial transient phase) while configurations (ii), (iii) and (iv) are taken either within the scaling regime (i.e. where $\sim t^{1/3}$ for $\lambda = 0$ and $t^{3/5}$ for $\lambda > 0$) or within the final slower-growth regime, especially the ones at late times for high values of $\lambda$.

As mentioned in the main text, domain morphology exhibits considerable differences for increasing values of $\lambda$. More specifically, for $\lambda \lesssim 10^{-3}$ (Fig. S3(a) and (b)) small-size domains (i) grow over time and form elongated structures (ii) which, due to coalescence and ripening, further coarsen (iii, iv) finally yielding large domains either rounded or perfectly circular. Note that the polarization displays a rather uniform orientation without topological defects, whose presence could be favored, for example, by imposing a preferential orientation of $\boldsymbol{p}$ at the fluid interface [11]. Note additionally that, within the domains, $\phi \sim \phi_{eq} \sim 2.2$ and $p \sim p_{eq} \sim 1.1$, values in agreement with the equilibrium ones obtained in Sec. I B with the parameters defined in Sec. II. For these values of $\lambda$, domain morphology shows features essentially akin to the ones of a bicontinuous-like pattern of the passive model B in the binodal region [8, 12, 13], that would actually result if $\lambda = 0$ and $\boldsymbol{p} = 0$. This is also corroborated by the growing length $L(t)$ (see Fig. 2 of the main text) which scales as $\sim t^{1/3}$, typical of models with conserved order parameter [8, 14–16].

For $\lambda > 10^{-3}$, the advective term $\lambda\nabla\cdot(\boldsymbol{p}\phi)$ significantly affects the morphology. If $\lambda = 10^{-2}$ (Fig. S3), for example, small rounded domains, appearing soon after the initial transient phase (i), grow over time giving rise to large asymmetric polar aggregates (ii, iii) often exhibiting protrusion-like branches. Then, these domains progressively turn into stationary spherical droplets (iv). Note crucially that, while at an early stage the polarization shows a

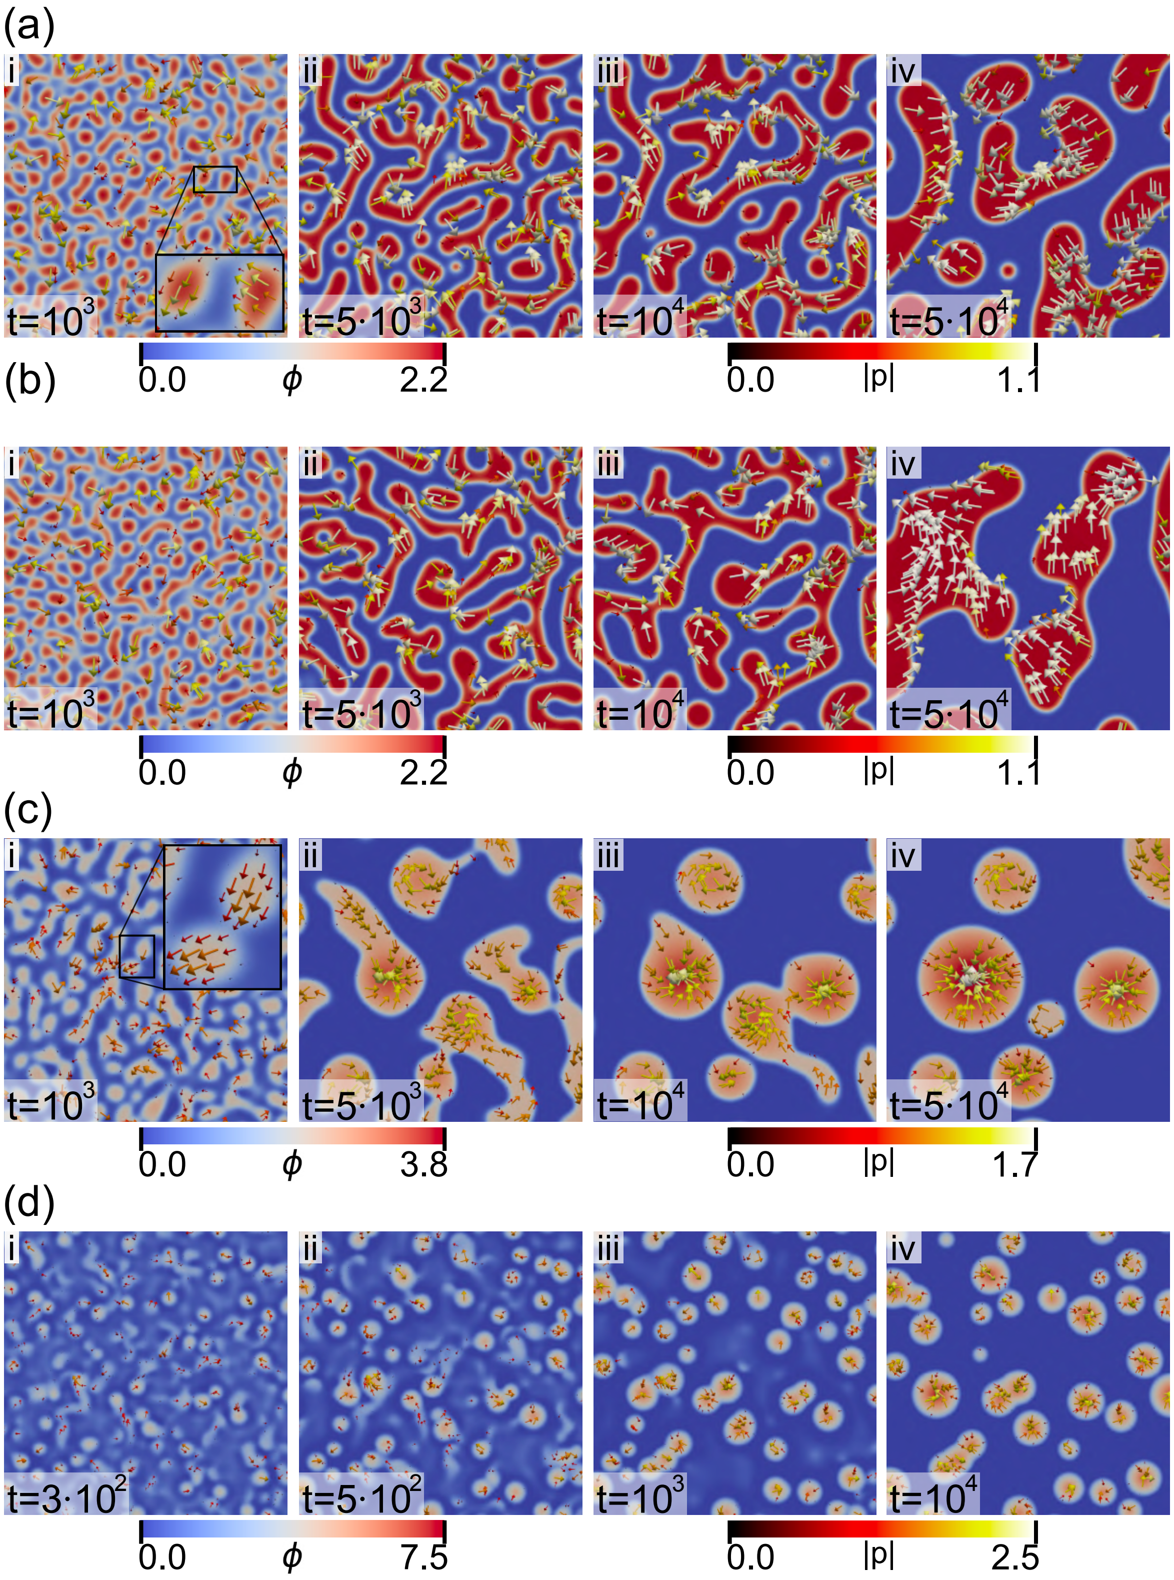


Figure S3. In this figure we show the time evolution of the active mixture for $\lambda = 10^{-4}$ (a), $\lambda = 10^{-3}$ (b), $\lambda = 10^{-2}$ (c) $\lambda = 10^{-1}$ (d) at different simulation times and for a portion of lattice of dimension $256 \times 256$ (the simulations are run on a square lattice of linear size $N = 512$). In panels (i) of (a) and (c) we also show a zoom of two rounded domains where the polarization is everywhere almost uniform and unidirectional. Parameter values are given in Section II A. Density and polarization range according to the corresponding color bars.

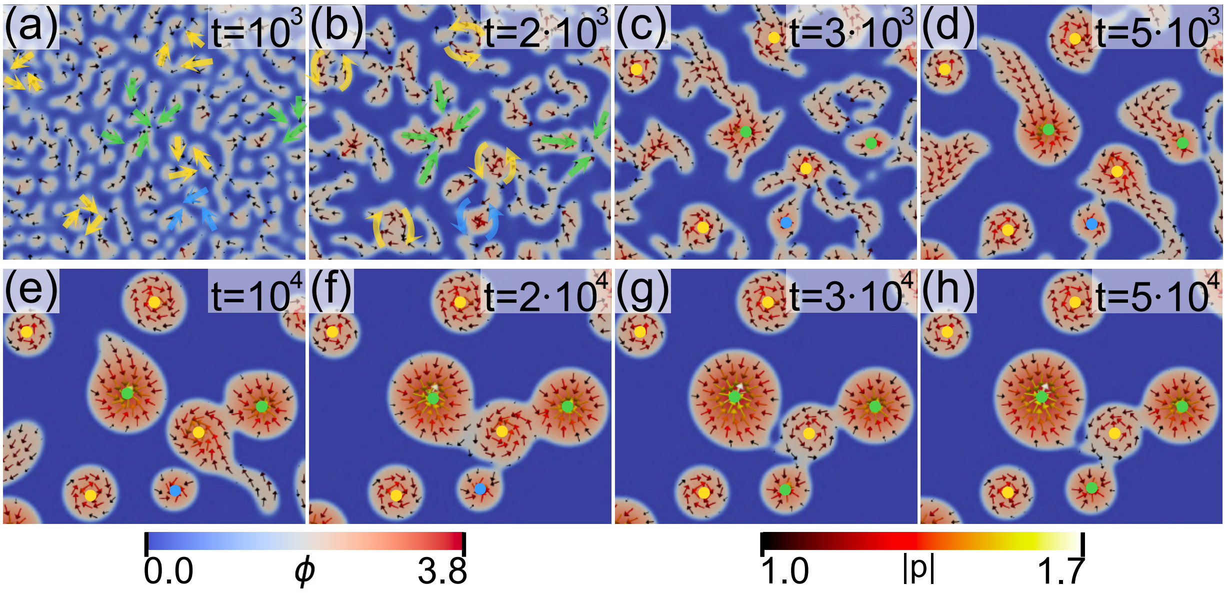


Figure S4. Morphological evolution of the system for $\lambda = 10^{-2}$, where configurations are taken at time intervals shorter than those shown in Fig. S3. Green, blue and yellow arrows in panels (a) and (b) denote the direction of motion of small domains which, once merging, originate inward aster-like, spiral-like and vortex-like defects, respectively. Green, blue and yellow dots highlight these defects, which are identified and located following the procedure described in Sec. II B. Density and polarization range according to corresponding color bars.

uniform orientation (i) (overall akin to the case $\lambda < 10^{-3}$), at late times such a configuration is mainly found within protrusions while more complex structures emerge within circular domains, where $\boldsymbol{p}$ exhibits aster-like, spiral-like and vortex-like configurations (ii, iii, iv). The morphological evolution at $\lambda = 10^{-1}$ proceeds on a similar ground, although in this case domains are considerably smaller (see also Fig. S6(a)) and acquire a round shape with a defect in the interior already at an early stage. This is because the rapid formation of circular domains suppresses the presence of protrusions (which would yield contact and merging), finally favoring coalescence only for close domains and hindering a faster coarsening.

*Topological defects.* Clearly, topological defects play a crucial role at high advection strength. A more accurate inspection about their formation and dynamic behavior is shown in Fig. S4 for $\lambda = 10^{-2}$. At early times ((a) and (b)) small domains move along the direction set by the polarization, an effect that eventually leads to collision and coalescence. However, while the merging of two fluid domains results in a single domain where the orientation of $\boldsymbol{p}$ is uniform and intermediate between those of the pre-colliding droplets, the merging of three (or more) domains leads to a domain hosting topological defects of integer charge (see also Sec. III). More specifically, if domains approach and collide radially (i.e. $\boldsymbol{p}$ point towards a common center as highlighted in panels (a) and (b) by green arrows), an inward aster-like defect emerges. Alternatively, if domains collide tangentially, a vortex-like defect forms (see the blue arrows in (a) and b)), while spiral-like defects result from an intermediate collision dynamics (see yellow arrows in the same figure). At this stage of evolution (c), large domains (most of which contain a defect) of irregular shape survive while small ones have evaporated through ripening. Afterwards, protrusion-like structures with a uniform polarization propel along the direction of $\boldsymbol{p}$ and towards the defect core, finally yielding regular rounded-shaped domains. Clearly, the $\lambda$ term regularizes the domain shape while stabilizing the inner defect profile, as shown in panels (d)-(h) where a large domain hosting an aster defect (green dot) gradually becomes circular as the tail moves towards the core.

We also note that, in aster-like configurations, the inward radial polarization compensates advection effects while, in vortex-like ones, the polarization would favor the rotation of the domain (a combination of the two processes is observed for spiral configurations). However, neither transversal motion nor substantial shape change are observed.

*Shape regularization.* A quantitative assessment of the shape regularization caused by the advection is discussed in Fig. S5, where we show the area of domains $A(n,t)$ as a function of their perimeter $p(n,t)$ computed at the same simulation times of Fig. S3 and evaluated as detailed in Sec. II B. Here $n$ is an index counting the lattice nodes within and at the boundary of each domain. Although more refined counting approaches exist (such as the marching square algorithm [17]), we prefer a simpler and less computationally intensive procedure, considering that the average large dimension of the cluster mitigate estimation errors (of the order $\mathcal{O}(\Delta N^2)$ and $\mathcal{O}(\Delta N)$ for area and perimeter respectively).

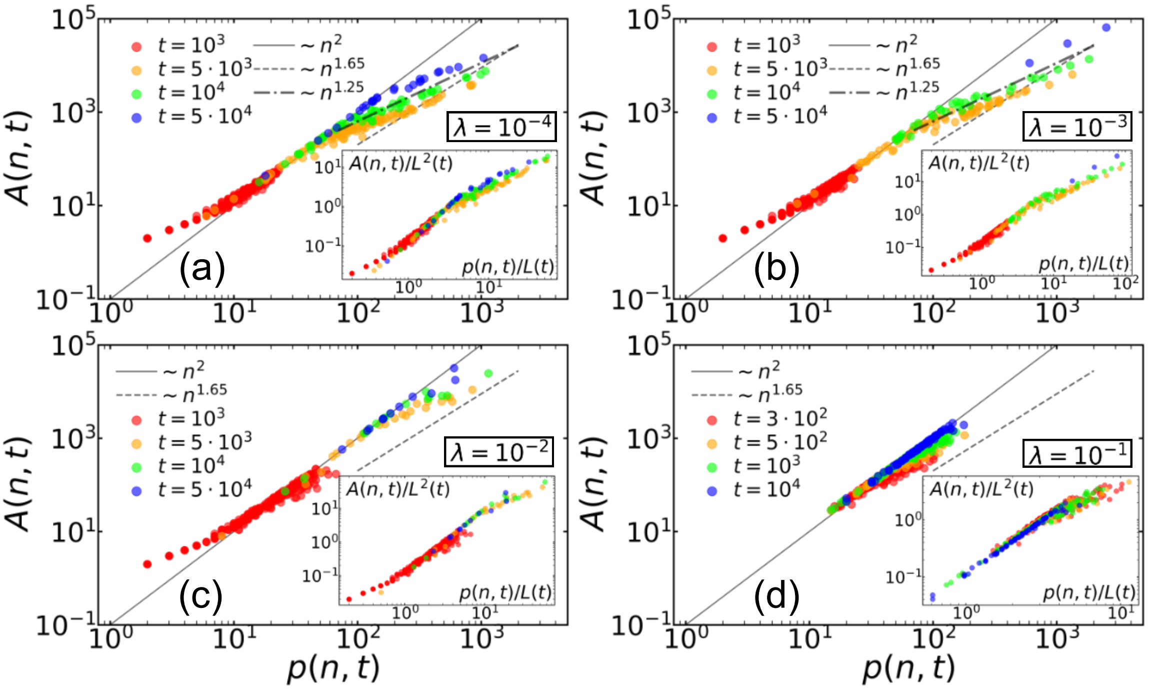


Figure S5. Area of domains $A(n,t)$ as a function of their perimeter $p(n,t)$ for systems with $\lambda = 10^{-4}$ (a), $\lambda = 10^{-3}$ (b), $\lambda = 10^{-2}$ (c) and $\lambda = 10^{-1}$ (d). In each panel, data are taken at the same simulation times of Fig. S3. Each datapoint refers to a single domain, while the continuous and dashed lines highlight the trends $\sim n^2$ and $\sim n^{1.65}$, respectively. In (a) and (b) the dot-dashed lines report the additional trend $\sim n^{1.25}$. Insets show data rescaled as $A(n,t)/L^2(t)$ vs $p(n,t)/L(t)$, with $L(t)$ the growing length from Fig. S6. The simulations parameters are the same as the ones in Fig. S3.

For a perfectly circular domain occupying $n$ lattice nodes, one would expect $A(n,t) \sim n^2$ and $p(n,t) \sim n$, thus the trend of $A(n,t)$ as a function of $p(n,t)$ is quadratic, as denoted by the black lines in all panels of Fig. S5. However, clear deviations from this trend are observed for $\lambda = 10^{-4}$ (a) and $\lambda = 10^{-3}$ (b) at late times, where irregular and elongated domains are present and yield a trend $\sim n^{1.25}$. Note, incidentally, that a lower-than-quatradic trend was found in molecular dynamics simulations of active dumbbells (see Fig. 11 in [18]), where $A \sim R_G^{1.65}$ with $R_G$ radius of gyration of the domains. For $\lambda = 10^{-2}$ (c) deviations are present only at early times, and a trend $\sim n^2$ is established afterwards. This is in agreement with the results shown in Fig. S4(c), where at late times only round domains are present. Finally, for $\lambda = 10^{-1}$ (d) the trend $\sim n^2$ dominates at all times since rounded domains rapidly form. We additionally note that all curves collapse on a common master curve when data are rescaled as $A(n,t)/L^2(t)$ vs $p(n,t)/L(t)$ (see the insets of Fig. S5), where $L(t)$ is the growing length from Fig. S6.

*Compression.* As mentioned in Sec. I, our model does not satisfy the incompressibility condition $\nabla \cdot \boldsymbol{p} = 0$, thus compression effects can emerge. This is the case shown in Fig. S3 and Fig. S4, where density and polarization of domains containing an inward aster-like or a spiral-like defect increase from the interface towards the bulk. On the contrary, domains with a vortex-like defect are characterized by a uniform density and polarization magnitude. This is the reason why, at very high values of $\lambda$ (such as $\lambda = 10^{-2}$), compression effects resulting from the aster-like polarization considerably decrease the domain size, decisively impacting the behavior of $L(t)$ (see Sec. V). For a more quantitative description we refer to Sec. VII, where we provide analytical estimates and trends of density values along with a functional form of the density profile close to the interface.

## V. THE GROWING LENGTH

In Fig. S6(a) we show an overview of the time evolution of $L(t)$ (defined in Sec. II A) for different values of $\lambda$ and $N = 512$, while in Fig. S6(b) $L(t)$ is computed for $N = 1024$. These results essentially provide a quantitative assessment of the morphological evolution discussed in the previous section.

For $\lambda < 10^{-3}$, the power-law trend $\sim t^{1/3}$ is attained once the initial transient phase (lasting up to $t \simeq 10^3$) is over. This is overall coherent with the fact that, for very low values of $\lambda$, our model approaches the passive model B, where

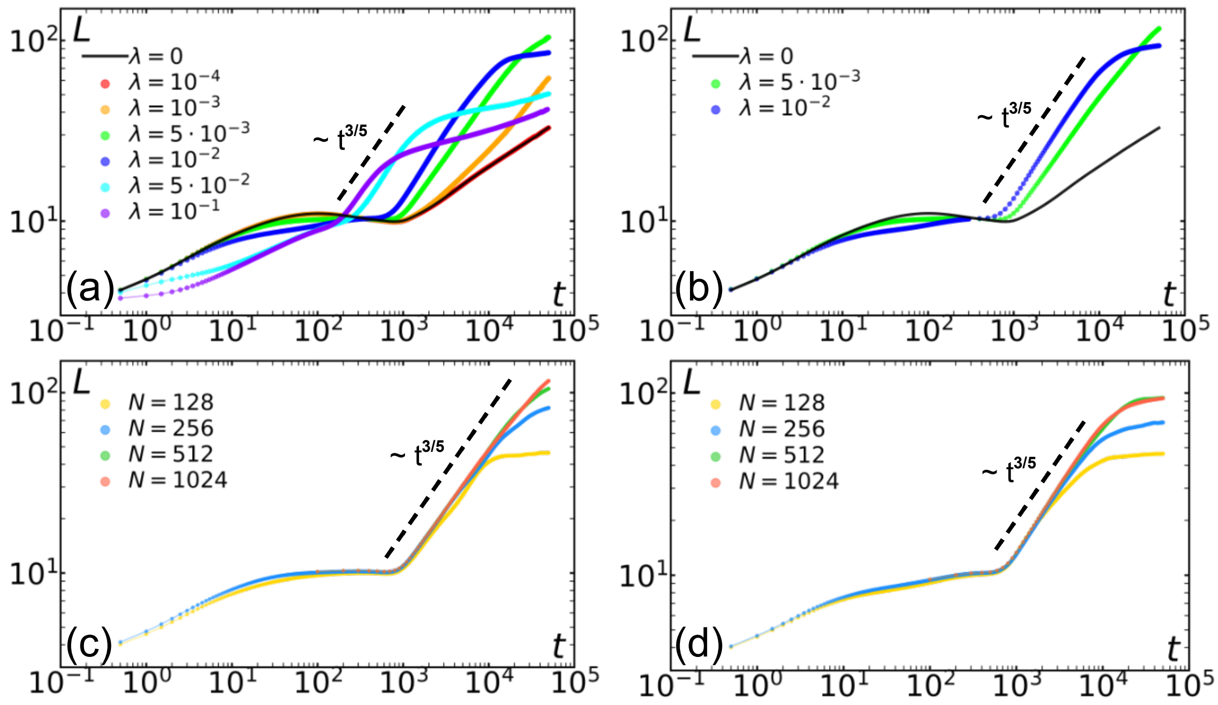


Figure S6. Time evolution of $L$ for different values of $\lambda$ and lattice size $N = 512$ (a) and $N = 1024$ (b). In (c) and (d) we show $L$ for $\lambda = 5 \cdot 10^{-3}$ and $\lambda = 10^{-2}$ respectively, and for different values of $N$. In all cases, the plots are averaged over 5 independent runs. The continuous lines shows a growth $\sim t^{1/3}$ while the dashed lines shows the $\sim t^{3/5}$ one. Other parameters are the same as those of Sec. II.

a diffusive scaling regime is found at late times [8, 16].

For increasing values of $\lambda$, domain coarsening occurs at a faster rate and a power-law regime $L(t) \sim t^{3/5}$ is clearly observed (Fig. S6(a)). Note that, at $\lambda = 10^{-3}$ where irregular and elongated domains are still observed (see also Fig. S3(b)), a crossover towards a $\sim t^{3/5}$ regime seems likely, although a well-defined power law within the time window under investigation can not be unambiguously established. As discussed in the main text, the reason of the faster growth at large $\lambda$ lies in the formation of integer topological defects (within domains resulting from colliding clusters) and the concurrent compression, an effect captured by the increase of density and polarization towards the center of domains containing aster-like and spiral-like defects (see also Sec. VIII). For $\lambda = 5 \cdot 10^{-3}$ and $\lambda = 10^{-2}$, at late simulation times (typically $t > 10^4$) $L(t)$ deviates from the $\sim t^{3/5}$ regime, a change that we interpret as due to a slower growth of circular isolated domains hosting integer defects (see also Fig. S4), rather than to finite size effects (see also Fig. S6(b), where a larger system is simulated). For higher values of $\lambda$ (such as $5 \cdot 10^{-2}$ and $10^{-1}$) similar considerations hold, although the $\sim t^{3/5}$ regime occurs earlier and lasts for shorter periods of time, essentially because of the rapid formation of circular domains finally leading to a dilute emulsion-like suspension.

Finally, in Fig. S6(c) and (d) we show $L(t)$ at large $\lambda$ and for values of $N$ ranging from 128 to 1024. Our results show that the regime $\sim t^{3/5}$ begins approximately at $t \sim 10^3$ in all cases, thus suggesting that the size of the system has negligible effects on the dynamics at early times. However, changing $N$ affects the time window of the $\sim t^{3/5}$ regime (which lasts longer for larger $N$) and, consequently, the beginning of the slower growth. Note that the curves obtained for $N = 512$ and $N = 1024$ overlap at late times too, thus suggesting, once again, that in this regime a mixture of immotile and isolated circular domains exhibiting a slower coarsening is eventually reached.

## VI. STRUCTURE FACTOR AND DYNAMICAL SCALING

This Section is devoted to the analysis of the spherically-averaged structure factor $S(k, t)$ (associated to the density-density correlations) as defined in Eq. (11) and to the verification of the dynamical scaling hypothesis.

Let us consider the structure factor $S(k, t)$ first. In Fig. S7 we report the time-dependent spherically-averaged structure factor $S(k, t)$ computed over a square lattice of linear size $N = 512$ (first row) and $N = 1024$ (second row) for three different advection strengths in each column, $\lambda = 0$ in (a) and (d), $\lambda = 5 \cdot 10^{-3}$ (b) and (e), and $\lambda = 10^{-2}$

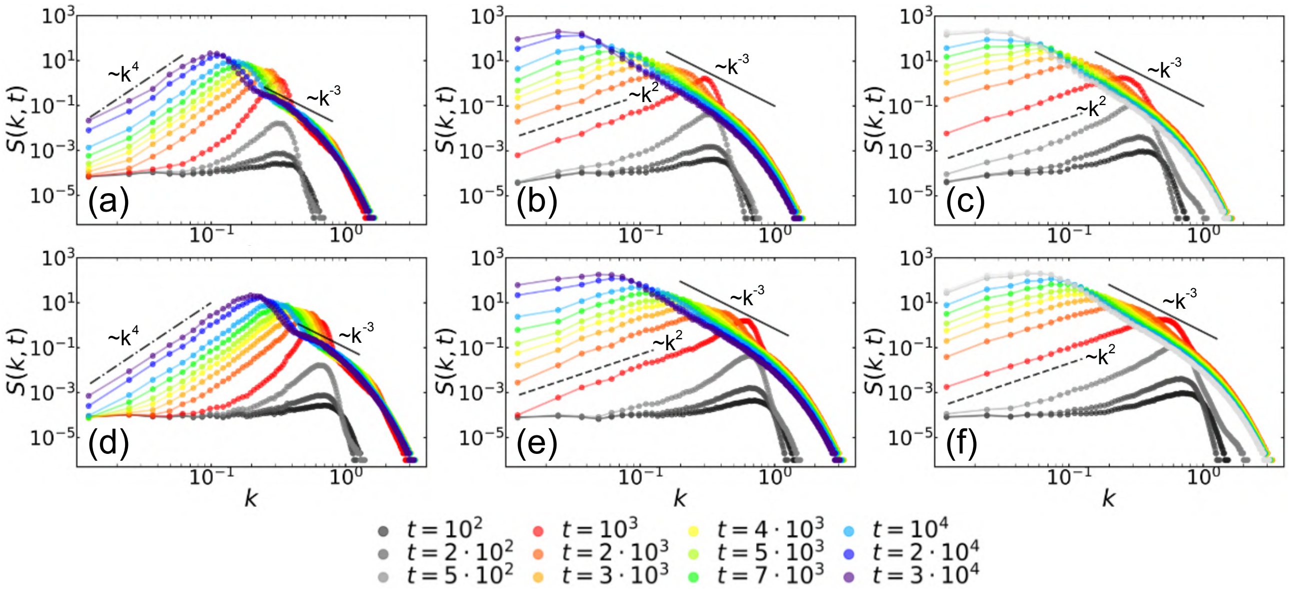

Figure S7. Time-dependent spherically-averaged structure factor $S(k,t)$ computed over a square lattice of linear size $N = 512$ with advection strength $\lambda = 0$ (a) $\lambda = 5 \cdot 10^{-3}$ (b) and $10^{-2}$ (c). Panels (d) to (f) show the behavior for the same values of $\lambda$ as in (a) to (c) for a larger system with $N = 1024$. The dot-dashed lines in (a) and (d) highlight the trend $\sim k^4$, while the dashed lines in all other panels highlight the trend $\sim k^2$. The black continuous lines in all panels report the Porod's law $\sim k^{-(d+1)}$ with $d = 2$. Data relative to times lower and larger than $t = 10^3$ are respectively colored in a gray and rainbow scale to remark that only after this time the growing regimes $\sim t^{1/3}$ or $\sim t^{3/5}$ are attained. In addition, in panels (c) and (f) the last two curves relative to $t = 2 \cdot 10^4$ and $t = 3 \cdot 10^4$ are colored in light gray to remark that with $\lambda = 10^{-2}$ at these times a slower-growth regime is observed. All other parameters are defined in Sec. II A.

in (c) and (f). In each panel, data are colored according to the legend at the bottom. Note that data relative to times lower and larger than $t = 10^3$ are respectively colored in a gray and rainbow scale. With reference to Fig. S6, this is to remark that only after this time the growing regimes $\sim t^{1/3}$ or $\sim t^{3/5}$ are attained. In addition, in panels (c) and (f) the last two curves relative to the two larger times $t = 2 \cdot 10^4$ and $t = 3 \cdot 10^4$ are colored in light gray to remark that with $\lambda = 10^{-2}$ at these times a slower-growth regime is observed.

As prescribed by Eq. (10), from the inverse of the first moment of the normalized structure factor $S(k,t)$ we estimate the time dependency of the growing length $L(t)$. In general, the increase in magnitude of the short wave-length peak as a function of time and its shift towards lower wave-vector values observed in all panels of Fig. S7 reflects the large scale ordering kinetics of the system. The case $\lambda = 0$ provides a benchmark, ensuring the well functioning of our numerical machinery. As expected and showed in Fig. S6, we indeed correctly estimate $L(t) \sim t^{1/3}$, not only for $\lambda = 0$, but also for $\lambda = 10^{-4}$. As suggested by [19], an alternative estimate of the growing length is provided by how the location of the peak of the structure factor $S(k,t)$ varies over time. The location of such a peak, which we denote as $\hat{k}(t)$, corresponds to the characteristic length scale in the system through the relation $\hat{L}(t) = \pi/\hat{k}(t)$. In Fig. S8(a) we report the trend of the growing length $\hat{L}(t)$ for the same $\lambda$ values as in Fig. S7. Here, curves were obtained using the trend of $S(k,t)$ sampled every 100 temporal units over a lattice of linear size $N = 1024$ and averaged over 5 independent runs (similar results are obtained for the case $N = 512$). In addition, we also applied a spline interpolation [20] to improve visualization. As expected, for $\lambda = 0$ also $\hat{L}(t)$ follows a $\sim t^{1/3}$ trend, while for the two larger $\lambda$ the trend $\sim t^{3/5}$ is once again observed.

As for the shape of $S(k,t)$, we remark that conservation of the order parameter typically reduces fluctuations at long wavelengths, i.e. at small $k$, and leads to $S(k,t) \downarrow 0$ for $k \downarrow 0$. The plots in Fig. S7 confirm this fact for all $\lambda$ (the points $S(0,t) = 0$ were correctly sampled but are not reported for visualization purposes). The way in which $S(k,t)$ falls off to zero for small $k$ depends, though, on $\lambda$. For $\lambda = 0$, Fig. S7 (a) and (d), the structure factor displays a $S(k,t) \sim k^4$ trend at small wave-vector, in agreement with the result from Furukawa concerning models where thermal fluctuations are not effective [15, 21]. The new non-trivial cases concern Fig. S7 (b), (c), (e) and (f) for $\lambda > 0$ (corresponding growing lengths $L(t)$ reported in Fig. S6), where data for long wavelengths are better described by $S(k,t) \sim k^2$. This seems to resonate with some of the comments from [15, 21], which state that such a trend at small $k$ is observed in systems where thermal fluctuations are instead effective. However, in our system there are no thermal fluctuations, so one could speculate that in presence of advection the morphology evolution detailed in Sec. IV could be actually occurring as if in presence of advective-related effects similar to thermal ones. For completeness, we recall that in

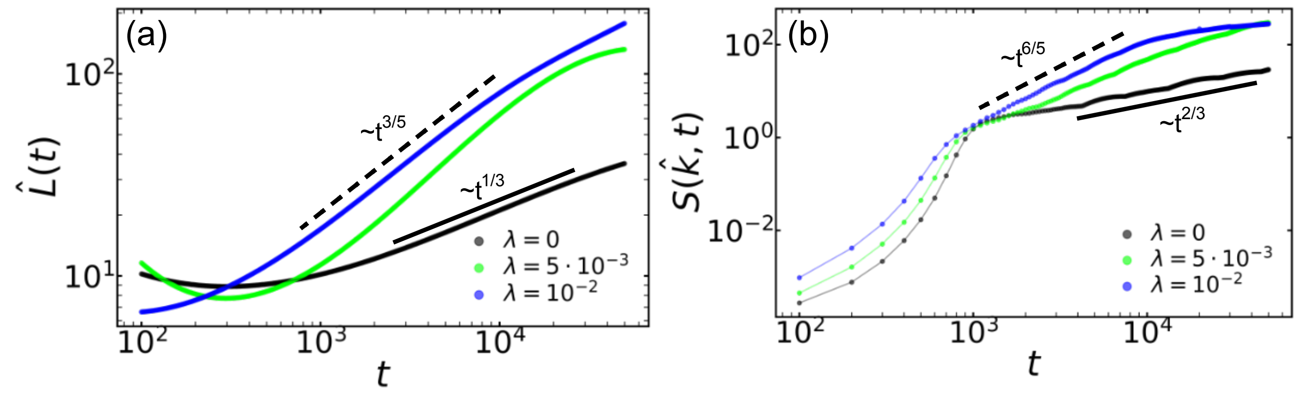


Figure S8. (a) Time trend of the growing length $\hat{L}(t) = \pi/\hat{k}(t)$, with $\hat{k}(t)$ location of the maximum of the structure factor $S(k,t)$, for the same $\lambda$ values as in Fig. S7. The continuous and dashed lines highlight the trends $\sim t^{1/3}$ and $\sim t^{3/5}$, respectively. (b) Time trend of the maximum of the structure factor $S(\hat{k},t)$ for the same $\lambda$ values as in Fig. S7. The continuous and dashed lines highlight the trends $\sim t^{2/3}$ and $\sim t^{6/5}$, respectively. In both panels, the parameters are $N = 1024$, $\phi_0 = 2$ ($\phi_{cr} = 1$), $M = 1$, $\alpha_\phi = 0.1$, $k_\phi = 0.5$, $\Gamma = 1$, $\alpha_{\boldsymbol{p}} = 0.1$, and $k_{\boldsymbol{p}} = 0.04$. (See Sec. II for details on the numerical integration and sampling methods), while curves were obtained using the trend of $S(k,t)$ sampled every 100 temporal units over a lattice of linear size $N = 1024$ and averaged over 5 independent runs. In (a), we also applied a spline interpolation [20] to improve visualization.

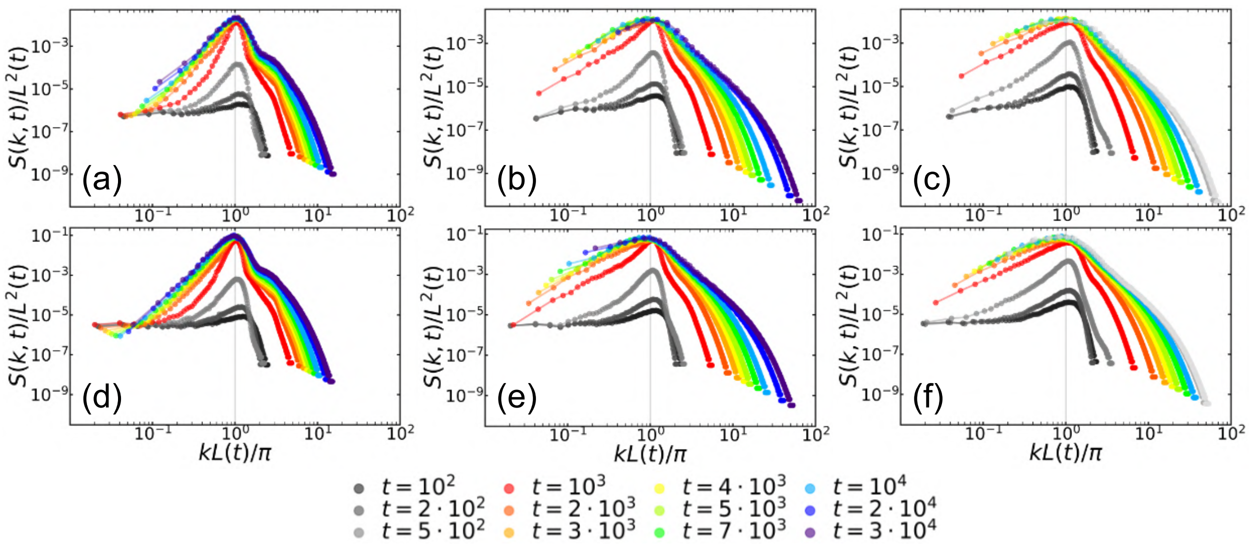


Figure S9. Test of the dynamical scaling hypothesis Eq. (19) for data relative to lattice linear size $N = 512$ and $N = 1024$ (rows) and three advection strengths $\lambda = 0$, $\lambda = 5 \cdot 10^{-3}$ and $\lambda = 10^{-2}$ (columns). For $S(k,t)$ we used the curves from Fig. S7 while for $L(t)$ the growing lengths from Fig. S6 extracted using Eq. (10). In Eq. (19) we fixed $d = 2$, while in all panels we plot the $k$-axis as $kL(t)/\pi$ so that the peak of the ratio $S(k,t)/L^d(t)$ is always located at $kL(t)/\pi = 1$, as hilighted by black vertical lines.

molecular dynamic simulations of Active Brownian Dumbbells (ABD), the structure factor in the small wavevector limit showed yet another trend, i.e. it was close to linearly dependent on $k$, $S(k,t) \sim k$ [18]. A better explanation and reconciliation of these different results calls for a deeper investigation. However, this is outside of the main scope of the present study, therefore we leave it for future studies. At larger $k$ (small scales), the structure factor typically exhibits a Porod's law [8, 22, 23], i.e. the structure factor shows the following power-law decay $S(k,t) \sim k^{-(d+n)}$ where $d$ is the spatial dimension and $n$ depends on the nature of defects and is equal to 1 for sharp domain walls, as in our case. The tails of the structure factor for $S(k,t) \gtrsim 0.1$ are in relative good agreement with this prediction, $k^{-3}$ (black segment in the plots), as occurred in [18] for ABD.

Let us now test the dynamical scaling hypothesis. According to [8], we briefly recall that the scaling hypothesis states that there exists, at late times, a single characteristic length scale $L(t)$ such that the domain structure is independent of time when lengths are scaled by $L(t)$. The existence of a single characteristic length implies that the

structure factor has the following scaling form

$$\frac{S(k,t)}{L^d(t)} = \mathcal{F}\left(kL(t)\right) \ , \tag{19}$$

where $d$ is the spatial dimension and $\mathcal{F}\left(kL(t)\right)$ is a scaling function which depends on the adimensional parameter $kL(t)$ and, although it can be different from system to system, does not vary over time time in intervals in which a dynamical scaling regime is attained. As a first test, we focus on the peak of the structure factor from Fig. S7, i.e. $S(\hat{k},t)$. In Fig. S8(b) we report the time trend of $S(\hat{k},t)$ for the same $\lambda$ values as in Fig. S7 and we observe that for $\lambda = 0$ the peak scales as $S(\hat{k},t) \sim t^{2/3}$, while for larger $\lambda$ as $\sim t^{6/5}$. Recalling that our system is two-dimensional, i.e. $d = 2$, and that $L(t)$ scales as $\sim t^{1/3}$ for $\lambda = 0$ and as $\sim t^{3/5}$ for larger $\lambda$ (see Fig. S6), we thus get that $S(\hat{k},t)$ correctly scales as prescribed by Eq. (19). As for the scaling of the entire structure factor $S(k,t)$, we refer to Fig. S9. Here, we extensively test the dynamical scaling hypothesis in our model plotting the ratio $S(k,t)/L^d(t)$ in different configurations and at different times. In particular, for $S(k,t)$ we use the curves from Fig. S7, with which Fig. S9 shares the same structure, while for $L(t)$ the growing lengths from Fig. S6 extracted using Eq. (10). In addition, we fix $d = 2$ in Eq. 19 and we plot the $k$-axis as $kL(t)/\pi$ so that, recalling that the peak of $S(k,t)$ is located at $\hat{k}(t)$ and an alternative measurement of the growing length is given by $\hat{L}(t) = \pi/\hat{k}(t)$, the peak of the ratio $S(k,t)/L^d(t)$ is always located at $kL(t)/\pi = 1$. Dynamical scaling is quite satisfactorily verified for sufficiently long times. Data collapse at late times allows us to define the *scaling regime* during which the dynamics fulfills Eq. (19). Interestingly, this seems to coincide with the time intervals during which $L(t)$ is observed to scale as $t^{1/3}$ ($t^{3/5}$) with $\lambda = 0$ ($\lambda > 0$). At early times up to when the growing regimes $t^{1/3}$ and $t^{3/5}$ begin, dynamical scaling is instead not satisfied, meaning that several length scales are still present in the initial growing kinetics.

## VII. STATIONARY DENSITY AND POLARIZATION PROFILES OF A SINGLE DROPLET

This Section focuses on a single spherical droplet with an inward aster-like polarization, as the ones displayed in Fig. S2(a) and Fig. S10(a).

In Sec. VII A we analyze the stationary configurations of density $\phi$ and polarization $\boldsymbol{p}$ within the droplet, but far from the interface. We show that the polarization compresses the mass and, consequently, the density profile is found to be not constant in the droplet interior. This effect was also qualitatively highlighted in the discussion of Sec. IV. We also determine the analytical dependency of the value of $\phi$ on radius $R$ and $\lambda$ at the center of the droplet, and show that the estimated results are in very good agreement with numerical simulations.

In Sec. VII B we complement our discussion by proposing an Ansatz for density and polarization profiles including regions at the interface and outside the droplet, and show that they accurately reproduce numerical profiles obtained in Sec. VII A.

### A. The stationary density and polarization profiles in the bulk

*Polarization profile of a droplet hosting an aster-like defect.* Given the spherical symmetry of the aster droplet, we use polar coordinates $(r,\theta)$ with $\phi \equiv \phi(r)$ and $\boldsymbol{p} \equiv (p(r), 0)$. From Eqs. (2) and (3), and using Eqs. (4) and (5), the stationary states are

$$M\nabla^2\mu_\phi - \lambda\nabla\cdot(\boldsymbol{p}\phi) = 0 \ , \tag{20}$$

$$\alpha_{\boldsymbol{p}}|\boldsymbol{p}|^2\,\boldsymbol{p} - \alpha_{\boldsymbol{p}}(\phi-1)\boldsymbol{p} - k_{\boldsymbol{p}}\nabla^2\boldsymbol{p} = 0 \ . \tag{21}$$

Let us first consider a region $r > r_c$ outside the defect core (which is the area of radius $r_c$ around the droplet centre where polarization magnitude varies from vanishing to peak value, see Fig. S11(c)) and far from the interface. The latter is positioned at distance $R$ defined as the maximum distance, from the centre of the droplet, where $\phi(r) \geq \phi_{eq}$ (see Sec. I B and the main text). Note that the configurations of the polarization found numerically (see Fig. S11(c)) show that the defect core typically spans over a limited area, thus $r_c$ can be considered equal to a few lattice nodes. Also, the thickness of the interface, where the density falls from typical values ($\geq \phi_{eq}$) inside the droplet to vanishing ones outside, is much smaller than $R$ (see Fig. S10(a)).

In the region $r_c < r < R$, the polarization $p(r)$ varies smoothly along the radial direction, thus it is reasonable to neglect the term $k_{\boldsymbol{p}}\nabla^2\boldsymbol{p} \sim 0$. This is also confirmed by Fig. S10(b), in which we show the (absolute value) of the

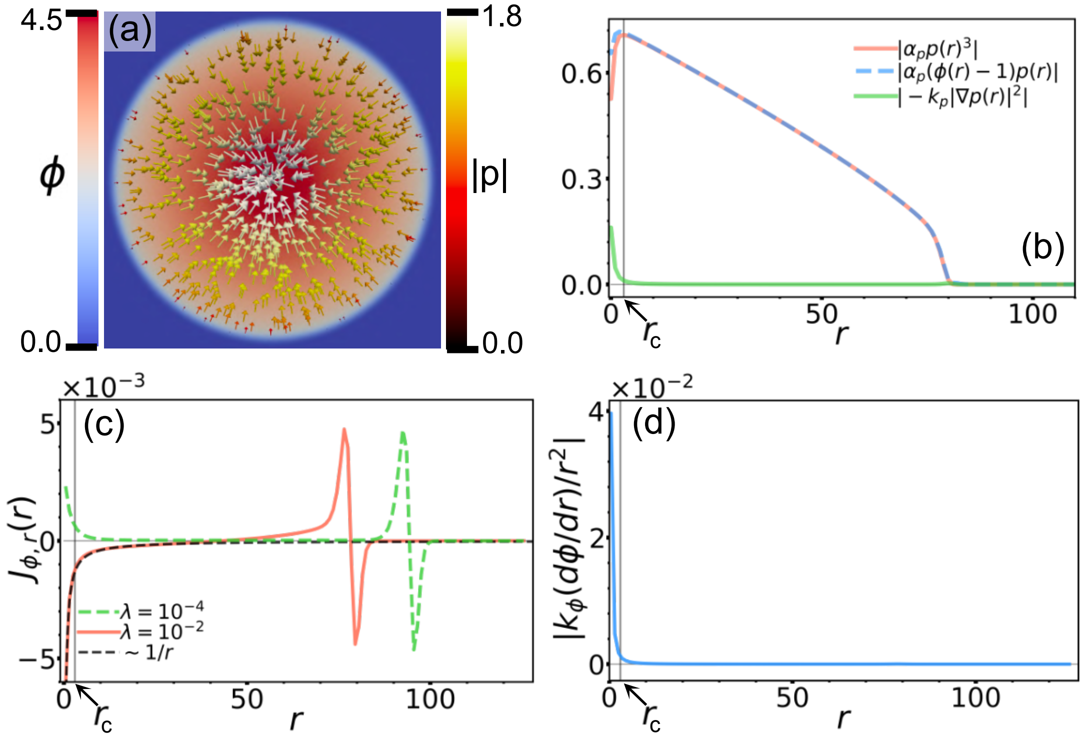


Figure S10. (a) Snapshot of a droplet with an inward aster-like configuration, advection strength $\lambda = 10^{-2}$ and equilibrium radius $R \sim 80$. Density field and modulus of the polarization vector are colored according to their respective color bars. (b) Absolute value of the three contributions from Eq. (21) relative to the droplet in (a). (c) Numerical estimate of the radial current $J_{\phi,r}(r)$ obtained from numerical simulations of a droplet with an inward aster-like configuration and two advection strengths, $\lambda = 10^{-4}$ and $\lambda = 10^{-2}$. In both cases, the droplet was prepared with initial radius $R = 100$, as detailed in Sec. II A, and the droplet with $\lambda = 10^{-2}$ is the one shown in (a) after equilibration. The dashed line shows the trend $\sim 1/r$. (d) Trend of the absolute value of the term $k_\phi(d\phi/dr)/r^2$ from Eq. (28). In panels (b) to (d) the gray vertical lines denote the size of the core defect $r_c \sim 3$. All other parameters are given in Sec. II.

radial profiles of the three terms of Eq. (21) obtained numerically for the droplet in Fig. S10(a). As a result, we get

$$p(r) = 0 \qquad \text{and} \qquad p(r) = \pm\sqrt{\phi(r) - 1}\ . \tag{22}$$

The solution $p(r) = 0$ is valid outside the droplet, together with $\phi(r) = 0$. The solutions $p(r) = \pm\sqrt{\phi(r) - 1}$ hold inside the droplet and describe an outward and an inward aster-like configuration, respectively. In the following we consider $p(r) = -\sqrt{\phi(r) - 1}$, since we are interested in inward asters. We note that this solution is valid for $\phi(r) > 1$, thus it cannot be used close to the interface where the term $k_{\boldsymbol{p}}\nabla^2\boldsymbol{p}$ is not negligible.

*Stationary equation of the density within the droplet.* Now we focus on the behavior of $\phi(r)$ inside the droplet and far from the interface. We recall that the density equation can be recast as

$$\dot{\phi} = -\nabla \cdot \boldsymbol{J}_\phi = 0\ , \tag{23}$$

where $\boldsymbol{J}_\phi \equiv -M\nabla\mu_\phi + \lambda\boldsymbol{p}\phi$. In radial components ($\boldsymbol{J}_\phi(\boldsymbol{r}) = (J_{\phi,r}(r), 0)$), one has

$$\nabla \cdot \boldsymbol{J}_\phi = \frac{1}{r}\frac{d(rJ_{\phi,r}(r))}{dr} = \frac{1}{r}J_{\phi,r}(r) + \frac{dJ_{\phi,r}(r)}{dr} = 0\ , \tag{24}$$

which yields

$$J_{\phi,r}(r) = \frac{c_J}{r}\ , \tag{25}$$

with $c_J$ integration constant. Hence

$$(-M\nabla\mu_\phi + \lambda\boldsymbol{p}\phi)_r = -\frac{c_J}{r}\ , \tag{26}$$

where the subscript $r$ denotes the radial component.

If advection is absent ($\lambda = 0$) or negligible ($\lambda \ll 1$), inside the polar domains the density is constant with value $\phi = \phi_{eq} = (1+\sqrt{1+\alpha_p/(2\alpha_\phi)}/2) \sim 2.2$ (see Sec. I B and also Fig. S3(a) and (b)). Thus, $\mu_\phi$ is constant and $c_J \sim 0$ in $r_c < r < R$, as also confirmed by the green curve in Fig. S10(c) for a droplet with $\lambda = 10^{-4}$, where $J_{\phi,r}(r)$ is evaluated by numerically sampling the radial component of the two terms on the left-hand side of Eq. (26). For higher values of $\lambda$, $J_{\phi,r} \sim 1/r$. Fits on different sets of numerical data reveal that $c_J/r$ is very small. In Fig. S10(c) red curve, for example, $c_J \sim 10^{-3}$ for the droplet shown in Fig. S10(a) with $\lambda = 10^{-2}$. It is thus reasonable to assume that under stationary conditions $c_J/r \sim 0$ in $r_c < r < R$. The equation for $\phi(r)$ can then be approximated by

$$(M\nabla\mu_\phi - \lambda \boldsymbol{p}\phi)_r = 0 \; , \tag{27}$$

which, up to first derivatives, reads

$$\left[\alpha_\phi\left(3\phi(r)^2 - 6\phi(r) + 2 - \frac{\alpha_{\boldsymbol{p}}}{2\alpha_\phi}\right) + \frac{k_\phi}{r^2}\right]\frac{d\phi}{dr} + \frac{\lambda}{M}\phi(r)\sqrt{\phi(r)-1} = 0 \; . \tag{28}$$

For very low values of $\lambda$ ($\lambda \ll 1$), Eq. (28) is solved by $\phi(r) = \text{const}$, where the constant is given by the integration condition at any $r$ inside the droplet. For large values of $\lambda$, we note that elastic contributions proportional to $k_\phi$ can be neglected, as shown in Fig. S10(d) where $k_\phi(d\phi/dr)/r^2 \sim 0$ for $r_c < r < R$. Hence, we obtain

$$\frac{\left(3\phi^2(r) - 6\phi(r) + 2 - \dfrac{\alpha_p}{2\alpha_\phi}\right)}{\phi(r)\sqrt{\phi(r)-1}}\, d\phi(r) = -\frac{\lambda}{M\alpha_\phi}dr \; . \tag{29}$$

Integration of the right-hand side in the interval $(r > r_c, R)$ gives

$$-\frac{\lambda}{M\alpha_\phi}(R-r) \; , \tag{30}$$

while integration of the left-hand side gives

$$\int_{\phi(r)}^{\phi(R)} \frac{3\tilde{\phi}^2(r) - 6\tilde{\phi}(r) + c_\phi}{\tilde{\phi}(r)\sqrt{\tilde{\phi}(r)-1}}\, d\tilde{\phi}(r) = 2\left[(-4+\tilde{\phi}(r))\sqrt{\tilde{\phi}(r)-1} + c_\phi \arctan\left(\sqrt{\tilde{\phi}(r)-1}\right)\right]\Bigg|_{\phi(r)}^{\phi(R)} \tag{31}$$

where $c_\phi \equiv 2 - \alpha_{\boldsymbol{p}}/2\alpha_\phi$. Combining Eq. (30) and Eq. (31), and using $\phi(R) \sim \phi_{eq} \sim 2.2$, we get

$$(4-\phi(r))\sqrt{\phi(r)-1} - c_\phi \arctan\left(\sqrt{\phi(r)-1}\right) = -\frac{\lambda}{2M\alpha_\phi}(R-r) + (4-\phi_{eq}) - c_\phi \arctan\left(\sqrt{\phi_{eq}-1}\right) \; . \tag{32}$$

*Trend of the density peak at the centre of the droplet.* Although Eq. (32) was derived for $r > r_c$, we can extrapolate its trend up to $r = 0$ relying on the continuity of the fields and on the fact that compression effects occur at $r \sim 0$ too, where their impact is expected to be higher. Indeed, that this is the case is shown in Fig. S11(a), where black lines represent the density profile of droplets with inward aster-like defects, advection strength $\lambda = 10^{-2}$ and radius $R$ ranging from $\sim 10$ to $\sim 180$, while red dashed lines are the numerical solution of Eq. (32) for four droplets. Black and red curves compare very accurately up to $R$, while also showing that the maximum value of $\phi(r)$ is attained at the centre of the droplet. Fig. S11(b) shows the polarization magnitude profile $\sqrt{\phi(r)-1}$ obtained using data from Fig. S11(a), and validates our results from Eq. (22).

Evaluating Eq. (32) at $r = 0$, we obtain

$$(4-\phi_{max}(R))\sqrt{\phi_{max}(R)-1} - c_\phi \arctan\left(\sqrt{\phi_{max}(R)-1}\right) = -\frac{\lambda}{2M\alpha_\phi}R + (4-\phi_{eq}) - c_\phi \arctan\left(\sqrt{\phi_{eq}-1}\right) \; , \tag{33}$$

where the dependence on $\lambda$ is implicit and $\phi_{max}(R)$ is the value of $\phi(r)$ at the center of the droplet (i.e. at $r = 0$). The accuracy of Eq. (33) is evident from Fig. S11(a), where red and black lines overlap at $r = 0$. A further proof is provided in Fig. S12, where we compute of $f_l(R) \equiv (\phi_{max}(R) - \phi_{eq})\sqrt{\phi_{max}(R)-1} + c_\phi \arctan(\sqrt{\phi_{max}(R)-1})$, evaluated for different $\lambda$ using the values of $\phi_{max}(R)$ obtained numerically (see Fig. S13), and $f_r(R) \equiv \lambda/(2M\alpha_\phi)R - (4-\phi_{eq}) + c_\phi \arctan(\sqrt{\phi_{eq}-1})$, evaluated using the corresponding numerical estimates of $R$.

Since on the left hand side Eq. (33) the term $c_\phi \arctan(\sqrt{\phi_{max}(R)-1})$ is bounded while $(4-\phi(r))\sqrt{\phi(r)-1}$ is not, the dominant contribution is given by $\phi_{max}^{3/2}(R)$. Thus

$$\phi_{max}^{3/2}(R) \sim \frac{\lambda}{2M\alpha_\phi}R \; , \tag{34}$$

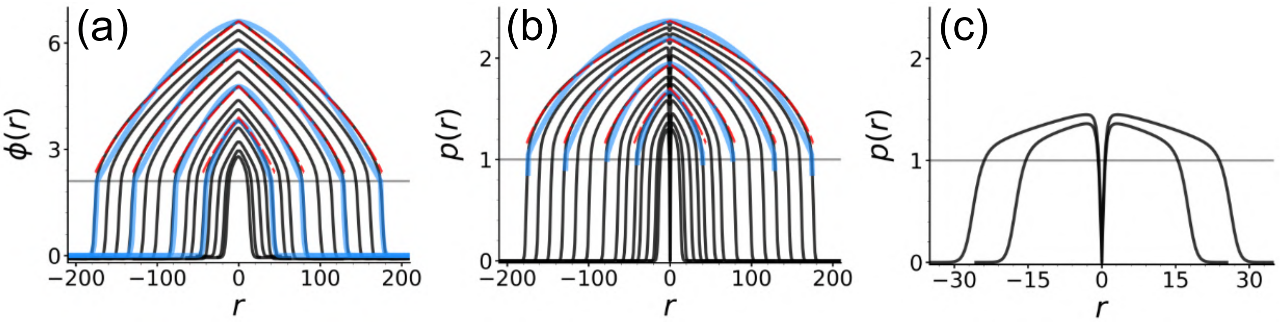


Figure S11. Figures (a) and (b) show density and polarization magnitude profiles along diameters of sample droplets with $\lambda = 10^{-2}$, inward aster-like polarization and radius $R$ ranging from $\sim 10$ to $\sim 180$. The black lines represent the numerical solution obtained from simulations while the red dashed curves show the numerical solution of Eq. (32) in (a) and the profiles $\sqrt{\phi(r) - 1}$ obtained from them in (b) for four sample droplets, up to $r \sim R$. The blue curves correspond to Eq. (42) with $c \sim 1.5$ and $\xi \sim 3$ and approximate the interface with the equilibrium expression for a scalar field theory. (c) Numerical profile $p(r)$ for droplets with radius up to $R \sim 30$, in which the lattice spacing is reduced to $\Delta N = 0.2$ to enhance the numerical resolution close to the defect core. All other parameters are given in Sec. II.

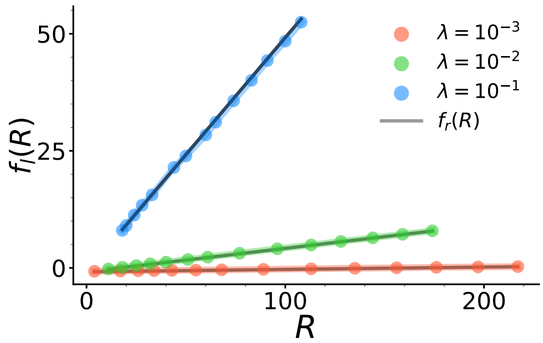


Figure S12. Numerical check of Eq. (33). Colored dots represent the left-hand-side $f_l(R) \equiv (\phi_{max}(R) - 4)\sqrt{\phi_{max}(R) - 1} + c_\phi \arctan(\sqrt{\phi_{max}(R) - 1})$ for different $\lambda$ evaluated using the $\phi_{max}(R)$ values obtained numerically and reported in Fig. S13. Black lines represent the right-hand-side, $f_r(R) \equiv \lambda/(2M\alpha_\phi)R - (4 - \phi_{eq}) + c_\phi \arctan(\sqrt{\phi_{eq} - 1})$, evaluated using numerical estimates of $R$.

where we dropped all constants on the right-hand side of Eq. (33). We finally get

$$\phi_{max}(R) \sim \left(\frac{\lambda}{2M\alpha_\phi} R\right)^{2/3} . \tag{35}$$

The above conclusion is tested in Fig. S13(a), where we report the trend of $\phi_{max}(R)$ obtained numerically for different advection strengths $\lambda$. Indeed, all curves for which $\lambda$ is large enough (i.e. $\lambda > 10^{-3}$) follow a $\sim R^{2/3}$ behavior. For $\lambda = 10^{-4}$, we instead observe that $\phi_{max}(R) \sim \phi_{eq} \sim 2.2$ for all $R$, consistent with the phenomenology of Model B without advection. Interestingly, Eq. (35) also shows that, at fixed $R$, $\phi_{max}(R)$ scales as $\sim \lambda^{2/3}$. This further conclusion is tested in Fig. S13(b), where data from Fig. S13(a) relative to $\lambda > 10^{-3}$ are rescaled as $(\phi_{max}(R) - \phi(R))/\lambda^{2/3}$, and a collapse on a master curve $\sim R^{2/3}$ is clearly noticeable.

*Polarization profile at the defect core.* To complete our analysis, we discuss possible solutions of Eq. (21) in the region $r < r_c$. In this region the term $k_{\boldsymbol{p}}\nabla^2 \boldsymbol{p}$ cannot be neglected, and Eq. (21) along the radial direction at stationarity becomes

$$\frac{d^2p(r)}{dr^2} + \frac{1}{r}\frac{dp(r)}{dr} + \frac{\alpha_{\boldsymbol{p}}}{k_{\boldsymbol{p}}}(\phi(r) - 1)p(r) = \frac{\alpha_{\boldsymbol{p}}}{k_{\boldsymbol{p}}} p^3(r) \qquad r < r_c . \tag{36}$$

This is a particular instance of a class of differential equations termed *non-linear Bessel equations* [24–26], whose analytical solution is beyond the scope of the present study. A numerical solution is shown in Fig. S11(b), where the profile of $p(r)$ is computed for different values of $R$ while at $\lambda = 10^{-2}$, and in Fig. S11(c) where the profile is shown for droplets with radius up to $R \sim 30$. Note the rapid dip in the region $r < r_c$, consistent with the location of a topological defect.

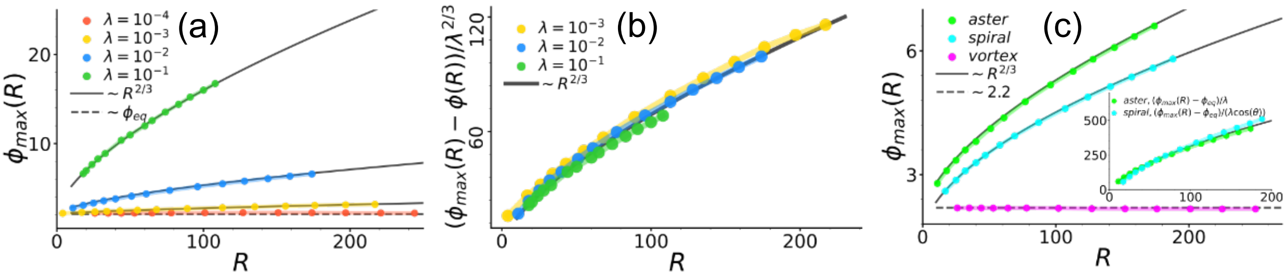


Figure S13. (a) Trend of $\phi_{max}(R)$ obtained from simulations of droplets with inward aster-like defects and increasing radius, for four different advection strengths $\lambda$. (b) Rescaling of the data shown in (a) as $(\phi_{max}(R)-\phi(R))/\lambda^{2/3}$ plotted against $R$. (c) Trends of $\phi_{max}(R)$ obtained from simulations of droplets with inward aster-like, spiral-like and vortex-like defects and increasing radius at $\lambda = 10^{-2}$. The spiral-like configuration is obtained for $\theta = \pi/4$. The inset reports the values of $\phi_{max}(R)$ for the aster-like and vortex-like cases from the main panel, rescaled as $(\phi_{max}(R) - \phi_{eq})/\lambda$ and $(\phi_{max}(R) - \phi_{eq})/(\lambda\cos(\theta))$. In all panels, black lines highlight the trend $\sim R^{2/3}$, while the dashed horizontal lines correspond to the value $\phi_{eq}$. All other parameters are given in Sec. II.

*Spiral-like and vortex-like configurations.* Finally, we briefly sketch how $\phi(r)$ and $p(r)$ change for inward spiral-like and vortex-like defects. A crucial difference with respect to an aster defect is that, in those cases, the advection strength takes an effective value $\lambda_{eff}$ such that $0 \leq \lambda_{\text{eff}} \leq \lambda$. This is because, although the polarization vectors contribute to advection, only the radial component of the polarization causes the compression. Aster and vortex defects represent two limiting cases. In the former, $\lambda_{\text{eff}} = \lambda$, and density and $\phi_{max}(R)$ have the profiles shown in Fig. S11 and Fig. S13. In the latter, $\lambda_{\text{eff}} = 0$, leading to flat density profiles and a constant trend for $\phi_{max}(R)$. Spiral-like configurations represent instead an intermediate case, in which the intensity of the advection strength is $\lambda_{\text{eff}} = \lambda\cos(\theta)$, where $\theta$ is an angle formed by the polarization vectors along the radial direction.

Quantitative support to the above discussion is provided by Fig. S13(c), in which we report the trend of $\phi_{max}(R)$ obtained from simulations of droplets with inward aster-like, spiral-like and vortex-like defects and increasing radius at $\lambda = 10^{-2}$. The spiral-like configuration is obtained by setting $\theta = \pi/4$. The figure clearly shows that the values of $\phi_{max}(R)$ of the spiral-like case are systematically lower than the ones of the aster-like case, while its functional form exhibits a $\sim R^{2/3}$ trend. In addition, $\phi_{max}(R) \sim \phi_{eq} \sim 2.2$ in the vortex-like configuration. A proof that advection strength scales as $\lambda_{\text{eff}} = \lambda\cos(\theta)$ is shown in the inset, where the values of $\phi_{max}(R)$ for the aster-like and vortex-like cases are rescaled as $(\phi_{max}(R) - \phi_{eq})/\lambda$ and $(\phi_{max}(R) - \phi_{eq})/(\lambda\cos(\theta))$ and are found to collapse on the same curve $\sim R^{2/3}$. Finally, the polarization of spiral-like droplets is akin to that of an aster droplet, while the one of vortex-like droplets exhibits a flat profile.

### B. Stationary profile including the interface

The analytical treatment presented in subsection VII A allowed us to estimate the profile not too close to the interface and the $\phi_{max}(R)$ dependency on $R$, which we have determined as the maximum distance from the centre of the droplet where $\phi(r) \geq \phi_{eq}$. However, a full analytical expression for the density profile $\phi(r)$ remains elusive. For this reason, here we propose the following Ansatz

$$\phi(r) = \theta(R-r)\left[a\left(\frac{r}{R}\right)^c + b\right] + \theta(r-R)\left[A + B\tanh\left(\frac{r-R}{\xi}\right)\right] \ , \tag{37}$$

where the first term on the right-hand side describes the profile inside the droplet, while the second one characterizes the interface and is inspired by the solution for flat interfaces in purely scalar models [8]. Here, $\theta(\pm R \mp r)$ denotes the Heaviside step function with the convention $\theta(0) = 1/2$, while $a, b, A, B$ are constants which we determine according to the following arguments:

- *Center of the droplet.* Eq. (37) reaches its maximum value $\phi_{max}(R)$ at $r = 0$, hence

$$\phi(0) = b = \phi_{max}(R) \ . \tag{38}$$

- *Interface.* At the interface, i.e. at $r = R$, Eq. (37) equals the interface value $\phi_{eq}$, hence

$$\phi_{eq} = \frac{1}{2}\left(A + a + \phi_{max}(R)\right) \qquad \Longrightarrow \qquad a = 2\phi_{eq} - \phi_{max}(R) - A \ . \tag{39}$$

- *Far away regions.* Outside the droplet, i.e. at $r \gg R$, the field vanishes, hence

$$\phi(r) = A + B \tanh\left(\frac{r-R}{\xi}\right) \underset{r\gg R}{\longrightarrow} A + B = 0 \qquad \Longrightarrow \qquad A = -B \ . \tag{40}$$

- *Continuity.* The two branches of Eq. (37) connect continuously at the interface, hence

$$\frac{A}{2} = \frac{2\phi_{eq} - \phi_{max}(R) - A + \phi_{max}(R)}{2} \qquad \Longrightarrow \qquad A = \phi_{eq} \ . \tag{41}$$

Putting all pieces together, we get

$$\phi(r) = \theta(R-r)\left[(\phi_{eq} - \phi_{max}(R))\left(\frac{r}{R}\right)^c + \phi_{max}(R)\right] + \phi_{eq}\ \theta(r-R)\left[1 - \tanh\left(\frac{r-R}{\xi}\right)\right] \ . \tag{42}$$

In the above expression, the parameter $c$ controls the concavity of $\phi(r)$ between 0 and $R$. Numerical evidence (see Fig. S11(a)) shows that $\phi(r)$ is concave, so $c > 1$. A more precise estimate of $c$ could be obtained by means of direct fits of the numerical profiles. However, we will see that the specific value of $c$ is not relevant for the growth argument presented in Sec. VIII.

The validity of the result in Eq. (42) as a good approximate solution for $\phi(r)$ in the full $r$ range is supported by two observations. First, in Fig. S11(a) we compare Eq. (42) plotted with $c \sim 1.5$ and $\xi \sim 3$ as blue lines with several sample numerical profiles, finding a good agreement between all curves. Second, we observe a posteriori that using Eq. (42) in Sec. VIII we get an estimate for the trend of $L(t)$ in good agreement with the one measured in the numerical solution of the full field equations.

## VIII. AN ARGUMENT TO EXPLAIN THE GROWTH OF $L(t)$

Here we present an argument to justify the enhanced growth of $L(t)$. Following the literature [8, 14], we refer to a circular droplet of radius $R(t)$, and we estimate how its radius varies over time. More precisely, our argument builds on the idea to balance the rate of change of mass of such a droplet with the dominant flux of mass over its surface. For the sake of simplicity, we assume as in [8] that the droplet evolves in a quasi-stationary fashion. In other words, we assume that the density field relaxes quickly compared to the rate at which the interface moves, and also that the density profile of the droplet is essentially the stationary one, so as to recover the results discussed in Sec. VII. This is consistent with visual inspection of configurations and also with the results from Fig. S6, where one can appreciate that domain size increases tenfold over the course of one or two decades. Before delving into our discussion, we remark that the calculations presented in the following aim at giving a reasonable explanation for the enhanced domain growth observed in Sec. V without being a rigorous proof for the value of the growth exponent.

As a preliminary benchmark of our approach, we first consider a circular droplet with radius $R$ evolving as prescribed by Model B, i.e. according to

$$\dot{\phi} = M\nabla^2\mu_\phi = -\nabla\cdot(-M\nabla\mu_\phi) = -\nabla\cdot\boldsymbol{J}_{\text{diff}} \ , \tag{43}$$

where $\boldsymbol{J}_{\text{diff}} \equiv -M\nabla\mu_\phi$ is the flux of mass through the droplet surface due to diffusion. The mass balance can be obtained by simply integrating Eq. (43) over the entire droplet surface, i.e.

$$\frac{d\mathcal{M}}{dt} = -\int_S \nabla\cdot\boldsymbol{J}_{\text{diff}}\ dS = -\oint_B (\boldsymbol{J}_{\text{diff}}\cdot\hat{n})\ dB, \tag{44}$$

where $S$ and $B$ respectively denote the droplet surface and its boundary, $\hat{n}$ denotes a versor everywhere normal to the latter, $\mathcal{M} \equiv \int_S \phi(x) d^2x$ denotes the total mass of the droplet and in the last step we used the divergence theorem. We now recall that in model B the density takes a constant value within the domains. Moreover, since radial symmetry holds, we have $\phi \equiv \phi(r)$ and $\boldsymbol{J}_{\text{diff}} \equiv (J_{\text{diff}}(r), 0) = (-M d\mu_\phi/dr)$. Therefore, the left-hand side of Eq. (44) is

$$\frac{d\mathcal{M}}{dt} \sim \frac{d}{dt}\int_0^R \phi(r)\ rdr \sim \phi_d \frac{dR^2}{dt} \sim R\frac{dR}{dt} \ , \tag{45}$$

where $\phi_d$ denotes the constant value of $\phi(r)$ within the droplet. The right-hand side becomes

$$\oint_B (\boldsymbol{J}_{\text{diff}}\cdot\hat{n})\ dB \sim M\frac{d\mu_\phi}{dr}\bigg|_R R \sim \frac{1}{R} \ , \tag{46}$$

where we used $d\mu_\phi/dr|_{r=R} \sim 1/R^2$, as prescribed by [8] for circular droplets. Putting all pieces together we finally get

$$R\frac{dR}{dt} \sim \frac{1}{R} \quad \rightarrow \quad \frac{dR^3}{dt} \sim 1 \quad \rightarrow \quad R \sim t^{1/3} \ , \tag{47}$$

i.e. the usual growth law $R \sim t^{1/3}$ typical of scalar models with conserved order parameter [8, 14–16].

Now we consider the effect of the advection. In this case, the dynamics are described by

$$\dot{\phi} = M\nabla^2\mu_\phi - \lambda\nabla\cdot(\boldsymbol{p}\phi) = -\nabla\cdot(-M\nabla\mu_\phi + \lambda\boldsymbol{p}\phi) = -\nabla\cdot\boldsymbol{J}_{\rm diff} - \nabla\cdot\boldsymbol{J}_{\rm adv} \ , \tag{48}$$

where $\boldsymbol{J}_{\rm diff} \equiv -M\nabla\mu_\phi$ represents the mass flux due to diffusion and $\boldsymbol{J}_{\rm adv} \equiv \lambda\boldsymbol{p}\phi$ is the flux due to advection. As a consequence, mass balance is now given by the following expression

$$\frac{d\mathcal{M}}{dt} = -\int_S \nabla\cdot\boldsymbol{J}_{\rm diff}\ dS - \int_S \nabla\cdot\boldsymbol{J}_{\rm adv}\ dS = -\oint_B (\boldsymbol{J}_{\rm diff}\cdot\hat{n})\ dB - \oint_B (\boldsymbol{J}_{\rm adv}\cdot\hat{n})\ dB \ . \tag{49}$$

In the following, we restrict our discussion to droplets with an inward aster-like configuration (as the one displayed in Fig. S2(a)) essentially becasuse, together with spiral-like defects, they outnumber vortex-like ones (see also Fig. 3 of the main text).

As discussed in Sec. VII, in the presence of advection the density profile is not uniform within the droplet, thus the scaling $\mathcal{M} \sim R^2$ has to be updated accordingly. Assuming that the density in the bulk can be described by the stationary profile given by Eq. (42), the total mass within a distance $r = R$ reads

$$\begin{aligned}\mathcal{M} &\sim \int_0^R \left[(\phi_{eq} - \phi_{max}(R))\left(\frac{r}{R}\right)^c + \phi_{max}(R)\right]\ rdr \\ &= \left[(\phi_{eq} - \phi_{max}(R))\ \frac{R^2}{c+2} + \phi_{max}(R)\frac{R^2}{2}\right] \\ &= \frac{2\phi_{eq} + c\phi_{max}(R)}{2(c+2)}R^2 \ .\end{aligned} \tag{50}$$

We remark that we use Eq. (42) since this is simple to integrate and captures the compression effects due to the advection. Using

$$\phi_{max}(R) \propto \left(\frac{\lambda}{M\alpha_\phi}\right)^m R^m \qquad \text{for} \ \ \lambda > 0 \ , \tag{51}$$

which generalizes Eq. (35) to a generic power $m$, the total mass within the droplet grows as

$$\mathcal{M} \sim \left(\frac{\lambda}{M\alpha_\phi}\right)^m R^{m+2} \ . \tag{52}$$

Note that we dropped the explicit dependency on the constant $c$ controlling the profile concavity and steepness, whose specific value, as anticipated in Sec. VII B, is not relevant for the growth argument developed here. As in Eq. (45), we now consider the time variation of $\mathcal{M}$ induced by the evolution of the radius of the droplet

$$\frac{d\mathcal{M}}{dt} \sim \left(\frac{\lambda}{M\alpha_\phi}\right)^m R^{m+1}\ \frac{dR}{dt}, \tag{53}$$

which reduces to Eq. (45) when $m = 0$ (i.e. for flat profiles).

Now we need to evaluate the scaling of the terms on the right-hand side of Eq. (49). Concerning the diffusion-related contribution, the formal steps shown in Eq. (46) are still valid, although now we have to consider the density profile given by Eq. (42). More specifically, using the chemical potential from Eq. (4), we get

$$\left.\frac{d\mu_\phi}{dr}\right|_{r=R} = \left[\left(\alpha_\phi(3\phi^2(r) - 6\phi(r) + 2) - \frac{\alpha_p}{2}\right)\frac{d\phi(r)}{dr} - k_\phi\left(-\frac{1}{r^2}\frac{d\phi(r)}{dr} + \frac{1}{r}\frac{d^2\phi(r)}{dr^2} + \frac{d^3\phi(r)}{dr^3}\right)\right]\Bigg|_{r=R} \ , \tag{54}$$

where we used $p(r) = -\sqrt{\phi(r) - 1}$, as prescribed by Eq. (22). From the expression of $\phi_{max}(R)$ given by Eq. (51), and noting that the derivative of order $n$ of Eq. (42) is

$$\left.\frac{d^n\phi}{dr^n}\right|_{r=R} = c(c-1)\cdots(c-n+1)\frac{(\phi_{eq} - \phi_{max}(R))}{R^c}r^{c-n}\Bigg|_{r=R} \sim \frac{\phi_{max}(R)}{R^n} = R^{m-n} \ , \tag{55}$$

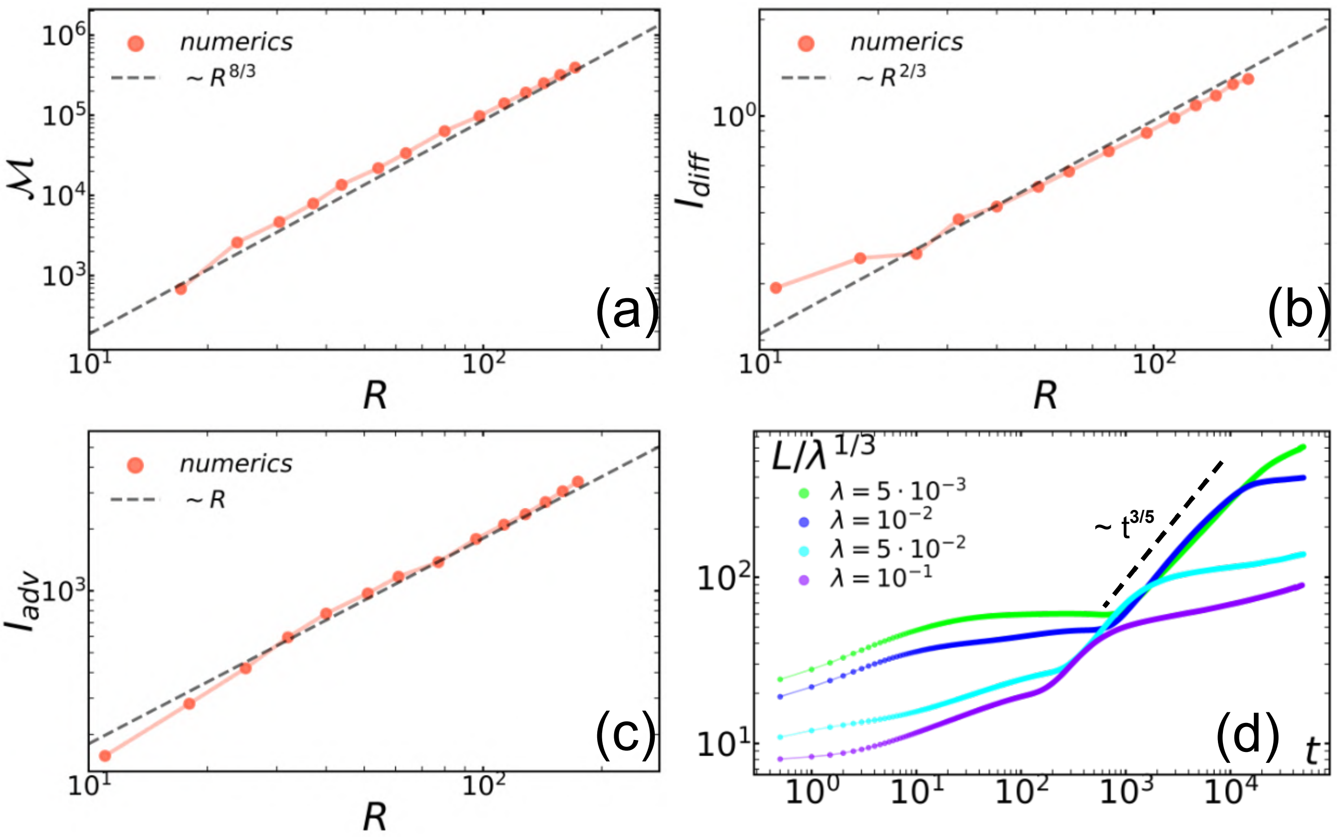


Figure S14. (a) $\mathcal{M} \equiv \int_0^R \phi(r)\ rdr$, (b) $I_{\rm diff} \equiv \int_0^R \nabla^2\mu_\phi\ rdr$ and (c) $I_{\rm adv} \equiv \int_0^R p(r)\phi(r)\ rdr$ evaluated from simulations of droplets with inward aster-like defects, increasing radius and $\lambda = 10^{-2}$. The dashed lines report trends $\sim R^{8/3}$ (a), $\sim R^{2/3}$ (b) and $\sim R$ (c). (d) Curves from Fig. S6(a) which present a $\sim t^{3/5}$ regime rescaled as $L/\lambda^{1/3}$. All other parameters are given in Sec. II.

we get, to leading order,

$$\left.\frac{d\mu_\phi}{dr}\right|_{r=R} \sim R^{m-1} \ , \tag{56}$$

thus

$$\oint_B (\boldsymbol{J}_{\rm diff} \cdot \hat{n})\ dB \sim M \left.\frac{d\mu_\phi}{dr}\right|_R R \sim MR^m \ . \tag{57}$$

This is different from the Model B where $d\mu_\phi/dr|_{r=R} \sim 1/R^2$. As for the advection-related contribution, we have

$$\oint_B (\boldsymbol{J}_{\rm adv} \cdot \hat{n})\ dB \sim \lambda R\phi(R)p(R) \sim \lambda R \ , \tag{58}$$

which vanishes when $\lambda = 0$.

From the above results it follows that the advection contribution becomes dominant over the diffusion one whenever $R_l \sim (\lambda/M)^{1/(m-1)}$. Although a precise estimate of $R_l$ would require a rigorous treatment of the above integrals, our result allows for some qualitative comments. Since in Sec. VII A we found $m \sim 2/3 < 1$ for circular droplets with inward aster-like configurations, we get $R_l \sim (M/\lambda)^3$, thus $R_l$ actually increases as $\lambda$ is decreased. This means that the smaller $\lambda$ is, the larger $R_l$ must be for the advective effects to dominate. This is consistent with the results reported in Sec. IV and Sec. V where we show that, for small $\lambda$, the evolution is driven by diffusion effects, with typical domain size growing as $L(t) \sim t^{1/3}$.

For the growing length $L(t) \sim t^{3/5}$ observed for larger values of $\lambda$, using once again the result $m \sim 2/3$ found in Sec. VII A, we get

$$\mathcal{M} \sim \left(\frac{\lambda}{M\alpha_\phi}\right)^{2/3} R^{8/3} \to \frac{d\mathcal{M}}{dt} \sim \left(\frac{\lambda}{M\alpha_\phi}\right)^{2/3} R^{5/3}\frac{dR}{dt} \ , \qquad \oint_B \boldsymbol{J}_{\rm diff}\cdot\hat{n} \sim MR^{2/3}, \qquad \oint_B \boldsymbol{J}_{\rm adv}\cdot\hat{n} \sim \lambda R \ . \tag{59}$$

These scaling laws are tested in Fig. S14, where we show that the dependence on $R$ of $\mathcal{M} \equiv \int_0^R \phi(r)\ rdr$, $I_{\rm diff} \equiv \int_0^R \nabla^2\mu_\phi\ rdr$ and $I_{\rm adv} \equiv \int_0^R p(r)\phi(r)\ rdr$ is reproduced, with good accuracy, by the respective trends obtained from Eq. (59). Since the dominant contribution comes from the advection, from Eqs.(49), (58) and (59) we finally get

$$\begin{aligned} \frac{d\mathcal{M}}{dt} &\sim \oint_B (\boldsymbol{J}_{\rm adv}\cdot\hat{n})dB \\ \left(\frac{\lambda}{M\alpha_\phi}\right)^{2/3} R^{5/3}\frac{dR}{dt} &\sim \lambda R \\ \frac{dR^{5/3}}{dt} &\sim \lambda^{1/3}(M\alpha_\phi)^{2/3} \\ R &\sim c_R t^{3/5}\ , \end{aligned} \tag{60}$$

where $c_R \equiv \lambda^{1/3}(M\alpha_\phi)^{2/3}$. In conclusion, when advection dominates over diffusion, our argument leads to $R \sim c_R t^{3/5}$, in agreement with $L(t) \sim t^{3/5}$ discussed in Sec. V. In Fig. S14(d) we also show that rescaling the curves of Fig. S6(a) as $L(t)/\lambda^{1/3}$ leads to a satisfactorily collapse on a curve $\sim t^{3/5}$.

## IX. MORPHOLOGY AND DOMAIN GROWTH IN GENERALIZED MODELS

Here we discuss a series of results obtained from extensions of the model presented in Sec. I. In particular, we study the effect of an additional advective contribution to the polarization equation, a generalized chemical potential to make contact with the framework of Active Model B, and an additional splay to the free energy. We limit our investigation to essential aspects of the morphology and domain growth, and to how the aforementioned modifications affect the scenarios emerged in Sec. IV and Sec. V. We anticipate that, even though the morphology and domain evolution may slightly differ from the ones described in Sec. IV, the overall results on domain growth described in Sec. V as well as the growth law $L(t) \sim t^{3/5}$ remain unaltered.

### A. Self-advection of the polarization

We start by considering the effect of an advective contribution to Eq. (3) proportional to $(\boldsymbol{p}\cdot\nabla\boldsymbol{p})\boldsymbol{p}$, so that the dynamics is now governed by the equations

$$\dot{\phi} + \lambda\nabla\cdot(\boldsymbol{p}\phi) = M\nabla^2\mu_\phi\ , \tag{61}$$
$$\dot{\boldsymbol{p}} + \Lambda(\boldsymbol{p}\cdot\nabla)\boldsymbol{p} = -\Gamma\boldsymbol{\mu_p}\ . \tag{62}$$

Note that these equations align to the more general framework of the Toner-Tu model from [27, 28]. The parameter $\Lambda$ in Eq. (62) controls the self-advective strength of $\boldsymbol{p}$ and resembles the familiar advective nonlinearity in the Navier-Stokes equation [29]. We remark that $\Lambda$ is a non-universal parameter determined by microscopic properties, thus $\lambda$ and $\Lambda$ do not necessarily take the same value, so that density and polarization can be advected at different speeds.

In order to give an idea of how this self-advection term alters the morphology described in Sec. IV, in Fig. S15 we show a set of configurations at increasing times for two values of $\Lambda$ and for $\lambda = 10^{-2}$. If $\Lambda = 10^{-3}$ (see Fig. S15(a) and Movie S3), the phenomenology is akin to that described in Sec. IV: small domains with uniform polarization initially form, and then collide and merge into larger domains while generating topological defects. The coarsening proceeds through further collisions finally leading to circular droplets. The relevant difference with respect to the dynamics shown in Fig. S3(c) is that, in this case, domains tend to maintain shapes curvilinear yet irregular and far from fully circular ones for longer times.

Increasing $\Lambda$ changes the scenario, as shown in Fig. S15(b) for $\Lambda = 10^{-2}$ (see also Movie S4). While at early times small domains survive, afterwards larger banana-shaped alongside pierced domains form. Their appearance can be traced back to the tendency of the polarization field to align approximately orthogonally and outwards to the interfaces. In particular, pierced domains are due to outward advection effects within domains of the dense phase, which result in the formation of bubbles of dilute phase within them, which in turn eventually reach the interface and mix with the background dilute phase (see Fig. S15(b)). As the system continues to evolve, domains eventually collide. Interestingly, when they impact in such a way that their polarizations approximately point toward a common collision point, bigger domains form with a polarization orthogonal to the interface but pointing inward. In particular, the

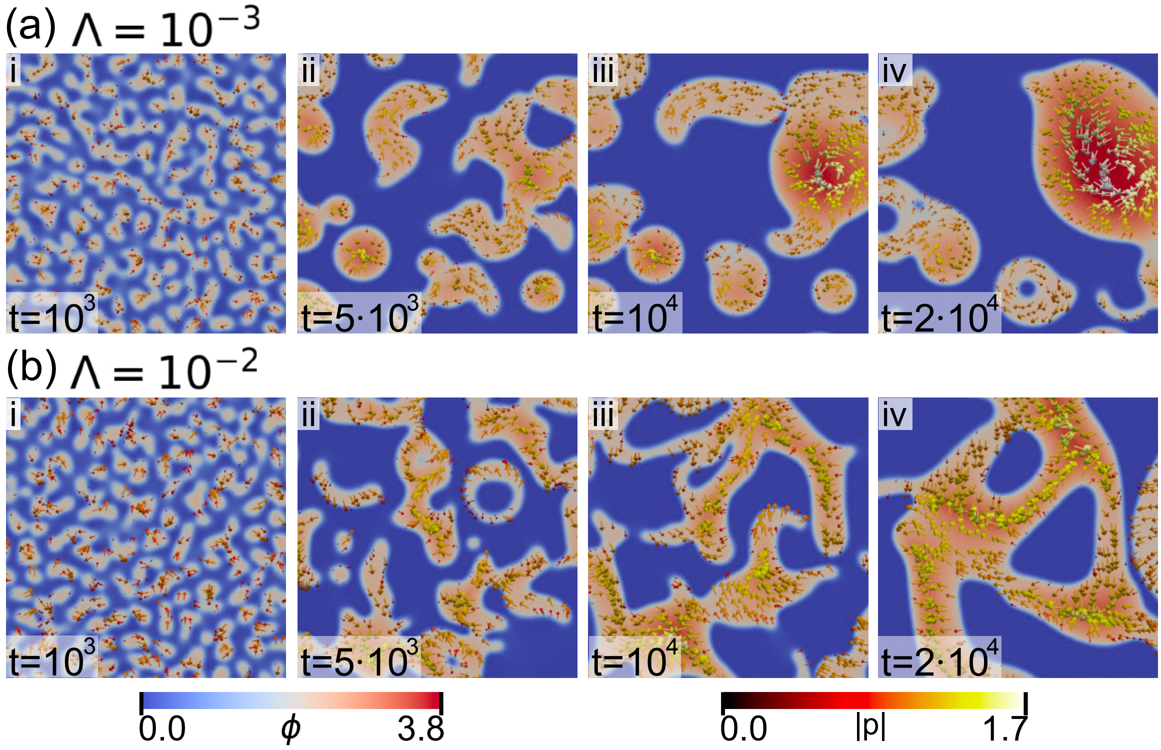


Figure S15. Model with advection on $\boldsymbol{p}$. Snapshots of an enlarged area of the system with $\lambda = 10^{-2}$, and $\Lambda = 10^{-3}$ (a) and $\Lambda = 10^{-2}$ (b). The density field and modulus of the polarization vector are colored according to the respective color bars. Simulations were run on a square lattice of linear size $N = 512$. The other parameters are given Sec. II.

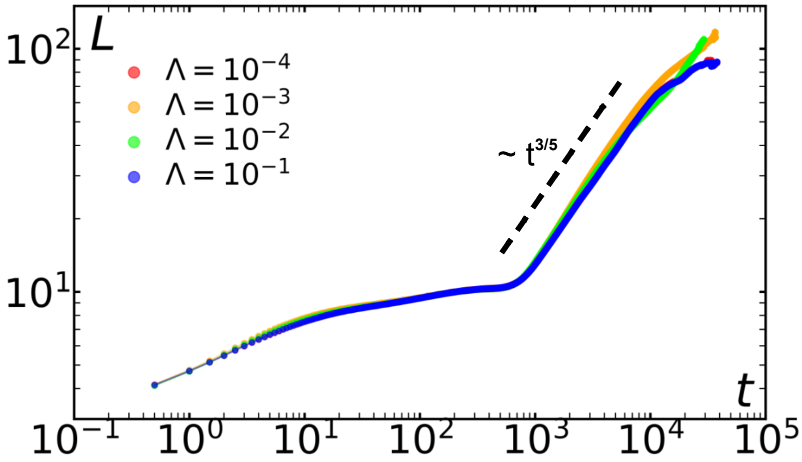


Figure S16. Growing length $L$ for $\lambda = 10^{-2}$ and different values of $\Lambda$. The dashed line shows the $\sim t^{3/5}$ behavior. Parameters are the same as in Fig. S15.

occurrence of regions where polarization pushes towards the interior of domains facilitates the formation of inward-pointing defects and the local increase of density. These regions are in turn connected by bridges where density and polarization are locally uniform.

These results suggest that, despite the non-trivial role played by $\Lambda$, the $L(t) \sim t^{3/5}$ regime holds (as shown in Fig. S16) and qualitatively confirm the arguments developed in Sec. IV and Sec. V.

### B. Contact with Active Model B

Active Model B (AMB) is a scalar field theory introduced in [30] to account, at a coarse-grained level, for the motility-induced phase separation, where active particles spontaneously phase-separate into dense and dilute phases in the absence of attractive interactions. Some features of this process can be modeled by introducing a leading-order square gradient term in the chemical potential violating detailed balance. In the present section, we aim to make contact with AMB by considering the following chemical potential

$$\mu_\phi = \frac{\delta F}{\delta \phi} = \alpha_\phi(\phi^3 - 3\phi^2 + 2\phi) - k_\phi \nabla^2 \phi - \frac{\alpha_p}{2}|\boldsymbol{p}|^2 + \zeta(\nabla\phi)^2 \ , \tag{63}$$

where the additional contribution $\zeta(\nabla\phi)^2$ is the one prescribed by [30] and $\zeta$ is the activity. Such active term breaks detailed balance in the usual Model B, thus the AMB cannot be derived from a free energy. The density and polarization equations given by Eq. (2) and Eq. (3) remain unaltered.

In previous works [30, 31] it has been shown that the active term yields a dispersion of droplets (akin to an asymmetric quench) growing over time with a power law $\sim t^{1/z}$, with $z$ dependent on the specific value of $\zeta$ and, in general, larger than the usual $z \sim 3$ from Model B.

In Fig. S17(a) we show the time evolution of the mixture with $\lambda = 10^{-4}$ and $\zeta = -1$, where droplets of the dense phase form in a dilute background. Since advection effects are negligible, we recover a phenomenology akin to that of the AMB sketched above, where droplets, here with uniform polarization, grow over time. In agreement with results from [30, 31], the coarsening proceeds at a slower pace than in Model B, with an estimated growth regime $\sim t^{0.25}$ ($z \sim 4$), as shown in Fig. S18(a). Similar results are obtained with $\zeta = 1$ (Fig. S18(b)), where in the initial regime droplets of the dilute phase are generated in a dense background.

For large values of $\lambda$ (see Fig. S17(b) and Movie S5 for $\lambda = 10^{-2}$ and $\zeta = -1$), advection becomes dominant and domain evolution shows features akin to those described in Sec. IV, where small domains collide and coalesce giving rise to large circular droplets hosting integer topological defects. Once again, we find that $L(t) \sim t^{3/5}$. For positive values of $\zeta$, similar considerations hold (see Fig. S17(c), Fig. S18(b) and Movie S6), albeit in this case the early stage of evolution is characterized by droplets of the isotropic phase immersed in a polar background. However, the large advection strength drives, once again, the formation of large polar domains through collision and merging, finally yielding circular polar droplets dispersed in an isotropic phase. We thus assist to a sort of inversion between dilute and dense regions, with the latter driving the domain evolution through collisions, merging and reshaping.

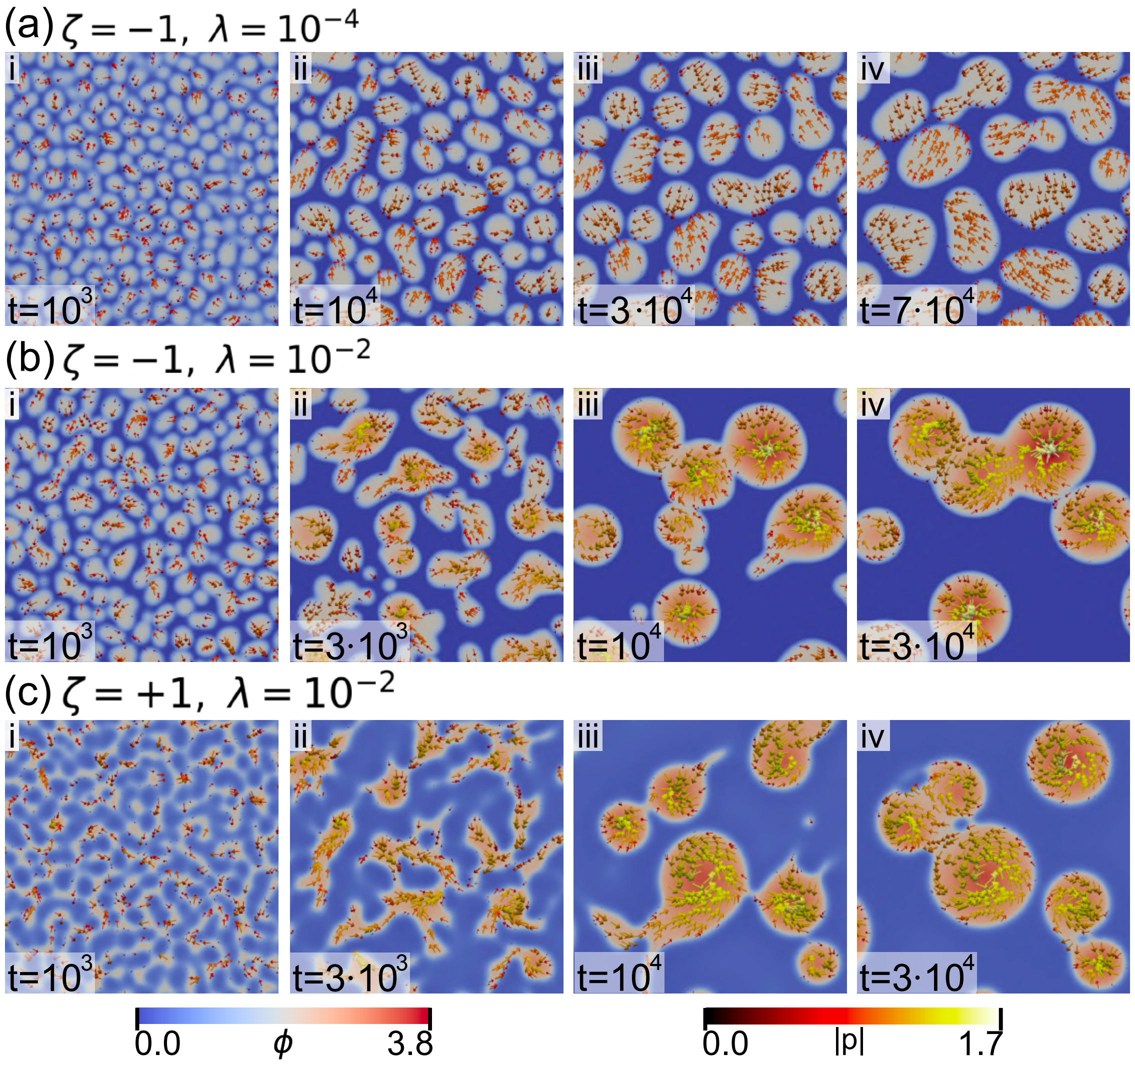


Figure S17. Extension to AMB. Snapshots of an enlarged area of the system with $\zeta = -1$ and $\lambda = 10^{-4}$ (a), $\zeta = -1$ and $\lambda = 10^{-2}$ (b), $\zeta = +1$ and $\lambda = 10^{-2}$ (c). Color bars indicate density and modulus of polarization. Simulations were run on a square lattice of linear size $N = 512$, while other parameters are the same as those given in Sec. II.

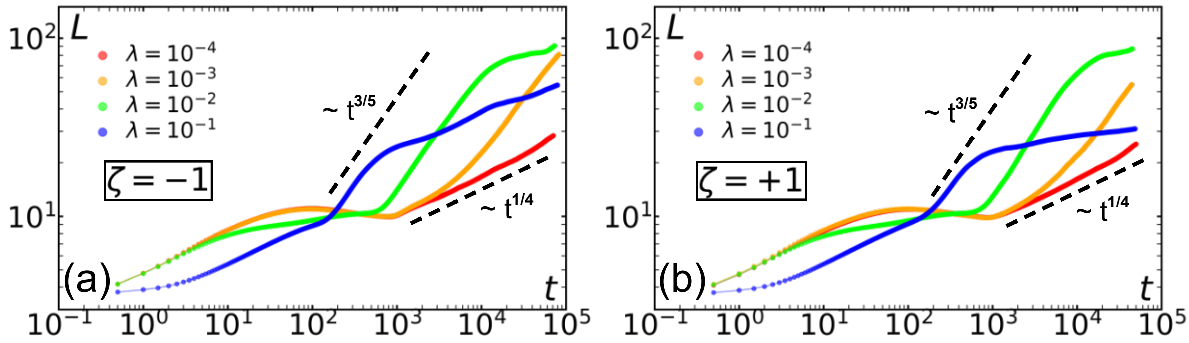


Figure S18. Growing length of the model extended to AMB. (a) Time-dependence of $L$ obtained with $\zeta = -1$ and $\zeta = +1$ for different values of $\lambda$. The dashed segments show the $\sim t^{1/4}$ and $\sim t^{3/5}$ behaviors. Simulations are run on a square lattice of linear size $N = 512$. Other parameters are given in Sec. II.

### C. Additional splay contribution

Finally, we investigate how domain coarsening changes when deformations of the polarization field are either favored or penalized. To pursue this goal, we consider the following modification to the free energy

$$F[\phi, \boldsymbol{p}] = \int d^2x \left\{ \left[ \frac{\alpha_\phi}{4\phi_{cr}} \phi^2 (\phi - \phi_0)^2 + \frac{k_\phi}{2} |\nabla \phi|^2 \right] + \left[ -\frac{\alpha_{\boldsymbol{p}}}{2} \frac{\phi - \phi_{cr}}{\phi_{cr}} |\boldsymbol{p}|^2 + \frac{\alpha_{\boldsymbol{p}}}{4} |\boldsymbol{p}|^4 + \frac{k_{\boldsymbol{p}}}{2} (\nabla \boldsymbol{p})^2 \right] + \omega (\nabla \cdot \boldsymbol{p})^2 \right\} , \quad (64)$$

where the additional contribution $\omega(\nabla \cdot \boldsymbol{p})^2$ either favors ($\omega < 0$) or penalizes ($\omega > 0$) total splay deformations [2].

If $\omega < 0$, the polarization in the domains would acquire an aster-like configuration, pointing either outwards or inwards. This is indeed shown in Fig. S19(a) (see also Movie S7), where we report a series of configurations at increasing times with $\lambda = 10^{-2}$ and $\omega = -10^{-2}$. We observe that, unlike the case shown in Fig. S4, here all domains are characterized by inward-pointing structures at late times, where the absence of aster pointing outwards depends on the mechanism of defect formation (resulting from the radial collision of domains, see Sec. IV). These results also suggest that the phenomenology is biased towards configurations featuring non-trivial density profiles due to compression effects. It is thus natural to expect that, in agreement with the arguments developed throughout the present work, the growth regime $L(t) \sim t^{3/5}$ still holds. This is shown Fig. S20(a), where for $\omega$ taking intermediate negative values such a regime is indeed present. Upon further augmenting $\omega$, splay effects become dominant, finally resulting in a null local advection. As a consequence, the system evolves as in the usual Model B, as shown in Fig. S19(b) for $\lambda = 10^{-2}$ and $\omega = -10^{-1}$, with a characteristic domain size growing as $L(t) \sim t^{1/3}$ (see Fig. S20(a)).

If $\omega > 0$, divergence-free configurations of the polarization, such as vortices, are promoted. This is clearly visible in Fig. S19(c) for $\lambda = 10^{-2}$ and $\omega = 10^{-2}$ (see also Movie S8), where no aster is present. However, for moderate (and positive) values of $\omega$, configurations featuring solely vortices are observed at late times, while at intermediate ones inward-pointing spirals are still present. Thus, as long as domains with non-flat density profiles survive, the growth regime $L(t) \sim t^{3/5}$ holds, as shown in Fig. S20(b).

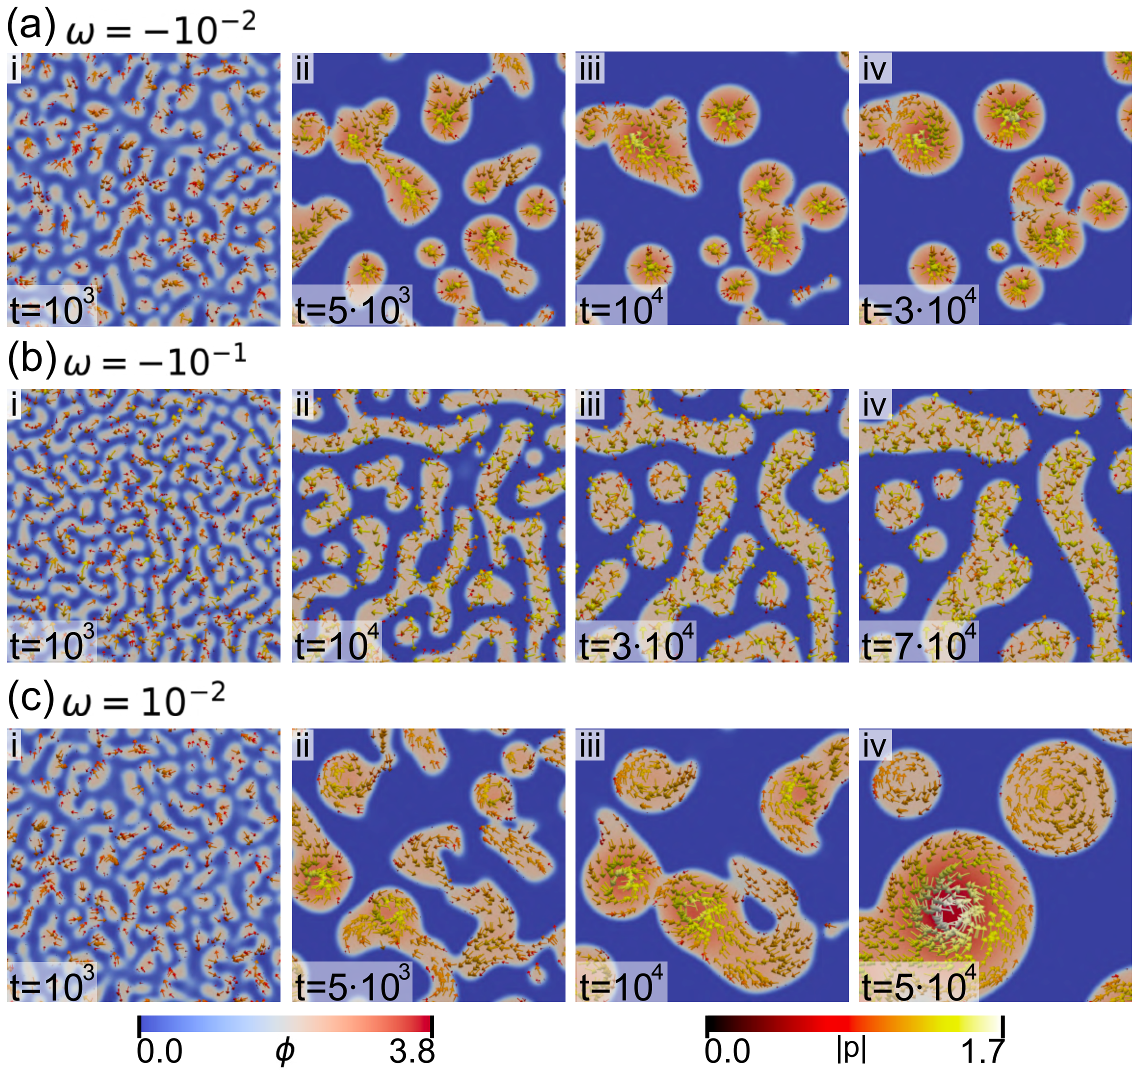


Figure S19. Additional splay contribution. Snapshots of an enlarged area of the system with fixed advection strength $\lambda = 10^{-2}$ and $\omega = -10^{-2}$ (a), $\omega = -10^{-1}$ (b), $\omega = 10^{-2}$ (c). Color bars refer to density and polarization field. Simulations are on a square lattice with linear size $N = 512$, while other are given in Sec. II.

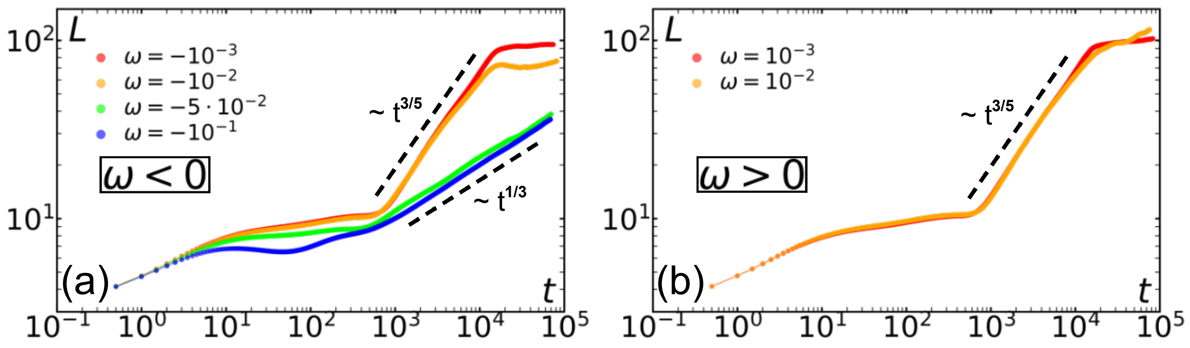


Figure S20. Growing length in the model with and additional splay contribution. The time-dependence of the growing length $L$ obtained with $\omega < 0$ and $\omega > 0$ with $\lambda = 10^{-2}$. The dashed line show the $\sim t^{1/3}$ and $\sim t^{3/5}$ behaviors. Other parameters are the same as those in Fig. S19.

## X. MOVIES

In the present section, we provide movies that illustrate the phase separation kinetics of our polar model in different configurations. They can be accessed online at https://www.dropbox.com/scl/fo/j6ire3bfn236jtxa9n1fz/AOeKJvu9gbO5Mpf_BhxQCd8?rlkey=xppwarj819csk5s8px3qmsy1r&st=izkfq12k&dl=0 and show the phase separation kinetics in the following cases:

- *Movie S1 and S2:* the original model described in Sec. I with advection strengths $\lambda = 10^{-4}$ and $\lambda = 10^{-2}$, respectively;

- *Movie S3 and S4:* the model from Sec. IX A, with an additional advective contribution in the polarization dynamics Eq. (3), advection strength $\lambda = 10^{-2}$ and self-advective strength $\Lambda = 10^{-3}$ and $\Lambda = 10^{-2}$, respectively;

- *Movie S5 and S6:* the model from Sec. IX B, with chemical potential Eq. (63) inherited from Active Model B, advection strength $\lambda = 10^{-2}$ and $\zeta = \mp 1$, which respectively favor the formation of droplets of a dense (dilute) phase in a dilute (dense) background;

- *Movie S7 and S8:* the model from Sec. IX C, with an additional splay contribution, fixed advection strength $\lambda = 10^{-2}$ and $\omega = \mp 10^{-2}$, which respectively favor aster and vortex configurations.

In all movies, all other parameters are given in Sec. II. For the sake of clarity, in the time intervals $[0,\ 10^3]$ (*initial regime*), $[10^3,\ 10^4]$ (*growth regime*) and $[10^4,\ 3 \cdot 10^4]$ (still *growth regime* in Movie S1, *final slower-growth regime* in all other Movies) movies show the system evolution with increasing speeds. Between *initial regime* and the central *growth regime*, Movie S1 and S2 show the evolution of an enlarged area of the system during the *growth regime*. In Movie S1 and S2 density and polarization are colored and range according to Fig. S3, while in Movie S3, S4, Movie S5, S6 and Movie S7, S8 according to Fig. S15, Fig. S17 and Fig. S19, respectively.

* massimiliano.semeraro@uniba.it
† adriano.tiribocchi@cnr.it

[1] J. W. Cahn and J. E. Hilliard, Free energy of a nonuniform system. I. Interfacial free energy, J. Chem. Phys. **28**, 258 (1958).
[2] P.-G. De Gennes and J. Prost, The physics of liquid crystals, 83 (Oxford University Press, 1993).
[3] L. N. Carenza, G. Gonnella, A. Lamura, G. Negro, and A. Tiribocchi, Lattice Boltzmann methods and active fluids, Eur. Phys. J. E **42**, 1 (2019).
[4] E. Tjhung, D. Marenduzzo, and M. E. Cates, Spontaneous symmetry breaking in active droplets provides a generic route to motility, Proc. Nat. Acad. Sc. **109**, 12381 (2012).
[5] R. J. LeVeque, Finite difference methods for ordinary and partial differential equations (SIAM, 2007).
[6] A. Frischknecht, Effect of shear flow on the stability of domains in two-dimensional phase-separating binary fluids, Phys. Rev. E **56**, 6970 (1997).
[7] A. Lamura and A. Tiribocchi, Shearing effects on the phase coarsening of binary mixtures using the active model B, Mathematics **9** (2021).
[8] A. J. Bray, Theory of phase-ordering kinetics, Adv. Phys. **43**, 357 (1994).
[9] V. M. Kendon, M. E. Cates, I. Pagonabarraga, J.-C. Desplat, and P. Bladon, Inertial effects in three-dimensional spinodal decomposition of a symmetric binary fluid mixture: a lattice Boltzmann study, J. Fluid Mech. **440**, 147 (2001).
[10] Scikit-learn Developers, DBSCAN - Density-Based Spatial Clustering of Applications with Noise (2025).
[11] F. Bonelli, L. N. Carenza, G. Gonnella, D. Marenduzzo, E. Orlandini, and A. Tiribocchi, Lamellar ordering, droplet formation and phase inversion in exotic active emulsions, Sci. Rep. **9**, 2801 (2019).
[12] P. C. Hohenberg and B. I. Halperin, Theory of dynamic critical phenomena, Rev. Mod. Phys. **49**, 435 (1977).
[13] S. Puri, Kinetics of phase transitions (CRC press, 2009) pp. 13–74.
[14] I. M. Lifshitz and V. V. Slyozov, The kinetics of precipitation from supersaturated solid solutions, J. Phys. Chem. Sol. **19**, 35 (1961).
[15] H. Furukawa, Effect of inertia on droplet growth in a fluid, Phys. Rev. A **31**, 1103 (1985).
[16] A. Onuki, Phase transition dynamics (Cambridge University Press, 2002).
[17] C. Maple, Geometric design and space planning using the marching squares and marching cube algorithms, in 2003 international conference on geometric modeling and graphics, 2003. Proceedings (IEEE, 2003) pp. 90–95.
[18] C. B. Caporusso, L. F. Cugliandolo, P. Digregorio, G. Gonnella, and A. Suma, Phase separation kinetics and cluster dynamics in two-dimensional active dumbbell systems, Soft Matter **20**, 4208 (2024).
[19] C. B. Caporusso, P. Digregorio, D. Levis, L. F. Cugliandolo, and G. Gonnella, Motility-induced microphase and macrophase separation in a two-dimensional active brownian particle system, Phys. Rev. Lett. **125**, 178004 (2020).
[20] C. De Boor and C. De Boor, A practical guide to splines, Vol. 27 (springer New York, 1978).
[21] H. Furukawa, Numerical study of multitime scaling in a solid system undergoing phase separation, Phys. Rev. B **40**, 2341 (1989).
[22] G. Porod, Die röntgenkleinwinkelstreuung von dichtgepackten kolloiden systemen: II. teil, Kolloid-Zeitschrift **124**, 83 (1951).
[23] H. Furukawa, A dynamical scaling assumption for phase separation, Adv. Phys. **34**, 703 (1985).
[24] Y. Kametaka, On a nonlinear Bessel equation, Publications of the Research Institute for Mathematical Sciences **8**, 151 (1972).
[25] J. W. Miles, On a nonlinear Bessel equation, SIAM J. Appl. Math. **42**, 109 (1982).
[26] N. T. Long, E. L. Ortiz, and A. P. N. Dinh, A nonlinear Bessel differential equation associated with Cauchy conditions, Comput. Math. Appl. **31**, 131 (1996).
[27] J. Toner and Y. Tu, Long-range order in a two-dimensional dynamical XY model: How birds fly together, Phys. Rev. Lett. **75**, 4326 (1995).
[28] E. Bertin, M. Droz, and G. Grégoire, Boltzmann and hydrodynamic description for self-propelled particles, Phys. Rev. E **74**, 022101 (2006).
[29] M. C. Marchetti, J. F. Joanny, S. Ramaswamy, T. B. Liverpool, J. Prost, M. Rao, and R. A. Simha, Hydrodynamics of soft active matter, Rev. Mod. Phys. **85**, 1143 (2013).
[30] R. Wittkowski, A. Tiribocchi, J. Stenhammar, R. J. Allen, D. Marenduzzo, and M. E. Cates, Scalar $\phi^4$ field theory for active-particle phase separation, Nat. Comm. **5**, 4351 (2014).
[31] S. Pattanayak, S. Mishra, and S. Puri, Ordering kinetics in the active model B, Phys. Rev. E **104**, 014606 (2021).
